# Supplementary material for: Field Theory of Bayesian Rate Estimation
Source: arXiv:2509.06129 source file (2026-09-23)
Supplement: Supplementary file 1 [file SM.tex]

\documentclass[%
 %reprint,
%superscriptaddress,
%groupedaddress,
%unsortedaddress,
%runinaddress,
%frontmatterverbose, 
%preprint,
%preprintnumbers,
%nofootinbib,
%nobibnotes,
%bibnotes,
 amsmath,amssymb,
 aps,
%pra,
%prb,
%rmp,
%prstab,
%prstper,
%floatfix,
]{revtex4-2}

\usepackage{graphicx}% Include figure files
\usepackage{dcolumn}% Align table columns on decimal point
\usepackage{bm}% bold math
\usepackage{cancel}
\usepackage{amsmath}
\usepackage{pgffor}

\DeclareMathOperator{\sign}{sgn}

%\usepackage{hyperref}% add hypertext capabilities
%\usepackage[mathlines]{lineno}% Enable numbering of text and display math
%\linenumbers\relax % Commence numbering lines

%\usepackage[showframe,%Uncomment any one of the following lines to test 
%%scale=0.7, marginratio={1:1, 2:3}, ignoreall,% default settings
%%text={7in,10in},centering,
%%margin=1.5in,
%%total={6.5in,8.75in}, top=1.2in, left=0.9in, includefoot,
%%height=10in,a5paper,hmargin={3cm,0.8in},
%]{geometry}

\begin{document}

\preprint{APS/123-QED}

\title{Supplementary Materials for the manuscript\\ ``Bayesian field theory of the rate estimation"}% Force line breaks with \\

%\author{Andrea Auconi}
 %\email{andrea.auconi@gmail.com}

%\author{Alessandro Codello}

%\author{Raffaella Burioni}

%\author{Guido Caldarelli}%

%

%

%\affiliation{%
 %Ca’ Foscari University of Venice, DSMN - via Torino 155, 30172 Mestre (Venice), Italy
%}%

%\date{\today}% It is always \today, today,
             %  but any date may be explicitly specified

\maketitle

\section{Bayesian rate estimation}

In the absence of a structural model for the dynamics of a phenomenon, and when the factors involved are multiple and uncertain, the framework of stochastic modelling is typically adopted \cite{karatzas1991brownian, risken1996fokker} and Bayesian theory \cite{petris2009dynamic} used for estimation.
In particular, when modelling a stochastic process which is known to be strictly positive, that is the case of a time-dependent rate of events $r\equiv r(t)$, the Geometric Brownian motion (GBM) is typically the minimal description employed. This process is written in the Ito interpretation \cite{karatzas1991brownian} as $dr = \sigma r \,dW $, where $dW$ are standard Brownian motion increments, and $\sigma$ the volatility parameter.

The Bayesian inference problem is to determine the probability of a particular realization of the stochastic process $r(t)$ given that a sequence of events $D\equiv \{ t^*_j \}_{j= 1, ..., n}$ has been observed.
This requires to specify a measurement model, which by the very definition of a rate is here given by the Poisson process, which defines the probability of observing an event in the time interval $[t, t+\Delta t)$ as asymptotically $r(t) \Delta t$ when $\Delta t \rightarrow 0$.
Field-theoretic approaches have been considered in \cite{chen2018density,nemenman2002occam,kinney2014estimation,kinney2015unification} following the seminal paper \cite{bialek1996field} for the Bayesian problem of estimating a 1D probability distribution from finite samples.
Here the problem is instead to derive a 1D rate function which has not got the normalization property of a probability. Nevertheless, the regularity properties considered in the mentioned field-theoretic approaches for a probability distribution can be equivalently described in the rate estimation setting by the path properties of Brownian motion or more general anomalous diffusions, as it was already observed in \cite{mora2019physical}.
Compared to Refs. \cite{mora2019physical, vergassola2007infotaxis, barbieri2011trajectories, auconi2022gradient} that consider the problem of filtering, that is to infer the current rate based on previous events, here in the study of historical time series of events the conditioning should include also events happened after any estimation time, as they will influence that time's rate estimate through the regularity assumptions on the underlying model dynamics.

\paragraph*{The free process.}
It is useful to consider the log-process $s\equiv \ln r$, whose dynamics is given by Ito Lemma as
$	ds = \frac{\partial s}{\partial r} dr + \frac{1}{2} \frac{\partial^2 s}{\partial r^2} dr dr = \sigma dW -\frac{\sigma^2}{2} dt $.
Given a time discretization $[t_0, t_1, ..., t_n]$ with $t_0=0$ and $t_n=T$ in the $n\rightarrow\infty$ limit of a vanishing time step $\Delta t \equiv T/n$, the probability density of a particular path $\boldsymbol{s}^{(n)} \equiv [s_0, ..., s_n]$ is written
\begin{equation}\label{A1}
	p_{\sigma}^{(n)}(\boldsymbol{s}^{(n)})
	= p(s_0)\prod_{i=1}^{n} p_{\sigma}(s_i|s_{i-1})
	 = p(s_0)\,(2\pi \Delta t)^{-\frac{n}{2}} \exp \left( - U_{\sigma}^{(n)}\left[\boldsymbol{s}^{(n)}\right] \right) ,
\end{equation}
where
\begin{equation}
    U_{\sigma}^{(n)}\left[\boldsymbol{s}^{(n)}\right] = f(\sigma) + \frac{s_n-s_0}{2} + \frac{\sum_{i=1}^{n}(s_i-s_{i-1})^2}{2\sigma^2 \Delta t} ,
\end{equation}
where $f(\sigma) \equiv n \ln \sigma  +\sigma^2 T/8$ is a term independent of the path accounting for the $\sigma$-specific normalization.
The explicit notation $p_{\sigma}\equiv p( \cdot |\sigma)$ with $\sigma$ on the subscript is to highlight that we are conditioning here on a particular value of the diffusion parameter. 
Please note that, while this probability density is defined over the space of all possible paths of any regularity, the actually observed realizations will have almost surely a quadratic variation of
\begin{equation}
    \lim_{n\rightarrow\infty}\sum_{i=1}^{n}(s_i-s_{i-1})^2 = \sigma^2 T,
\end{equation}
according to the Lévy characterization theorem \cite{karatzas1991brownian}. 
In principle we could model the initial value $s_0$ as a normally distributed $p(s_0)$ with mean $A$ and variance $B$. %= (2\pi A)^{-\frac{1}{2}} \exp\left[ -\frac{(s_0-B)^2}{2A} \right]
In practice, in the limit of a large rate of events close to the $t=0$ border this prior can be neglected as we will do in the following. Formally, this can be obtained by considering the limit $A\rightarrow \infty$.

The joint probability density of the path including its initial state can then be written as a Boltzmann distribution $p_{\sigma}^{(n)}(\boldsymbol{s}^{(n)}) = \exp\left(-U_{\sigma}^{(n)}[\boldsymbol{s}^{(n)}]\right) / \widetilde{Z}^{(n)}$, 
where $\widetilde{Z}^{(n)}$ is the prior normalization independent of $\sigma$.
Consider now a perturbation of the path $\boldsymbol{s}^{(n)}$ by the vector $\epsilon \boldsymbol{\phi}^{(n)}$. The first variation of the potential is
\begin{equation}\label{variation V}
    \partial_\epsilon U_{\sigma}^{(n)}[\boldsymbol{s}^{(n)}+\epsilon \boldsymbol{\phi}^{(n)}] |_{\epsilon=0} = \frac{\phi_n-\phi_0}{2} - \frac{\Delta t}{\sigma^2} \sum_{i=0}^{n} \phi_i (d_t^2 s)_i^{(n)},
\end{equation}
where the discrete Laplacian is defined as
$(d_t^2 s)_i^{(n)} \equiv (\Delta t)^{-2} (s_{i+1} +s_{i-1} -2 s_i)$ for $0<i<n$, with boundary conditions $(d_t^2 s)_0^{(n)} \equiv (\Delta t)^{-2} (s_{1} - s_0)$ and $(d_t^2 s)_n \equiv (\Delta t)^{-2} (s_{n-1} - s_n)$.

\paragraph*{Conditioning on sparse  events data.}

We now consider the Bayesian estimation of the time-dependent log-rate $s(t)$ based on the GBM prior and on a given realization of the events. The latter is the measured spike train $D\equiv (t_1, t_2, ..., t_m)$ of $m$ discrete events over the time interval $[0, T]$.
Assume the events to be generated from a rate-dependent Poisson process \cite{risken1996fokker}, meaning that the probability of observing a set of events $D\equiv (t_1, t_2, ..., t_m)$ from a particular profile of the rate curve $r(t)$ is
\begin{equation}
    p^{(n)}(D | \boldsymbol{s}^{(n)}) = \prod_{i=0}^{n} \left[ \mathbb{I}_{i \in D} r_i \Delta t + (1-\mathbb{I}_{i \in D}) (1-r_i \Delta t) \right] 
    \approx  (\Delta t)^{|D|} \exp \left[ \sum_{i \in D} s_i  - \sum_{i=0}^{n} e^{s_i} \Delta t \right],
\end{equation}
where $|D|$ is the total number of events, and $\mathbb{I}_{i \in D}$ is the indicator function being $1$ when there is one event in $D$ which lies in the $i$th interval of the time discretization, and $0$ otherwise. Note that implicitly also the discretization indices $r_i\equiv r_i^{(n)}$ and $s_i\equiv s_i^{(n)}$ are dependent on the discretization parameter $n$.
The effect of multiple events is negligible in the limit $\Delta t \rightarrow 0$, and also the sum over $i \notin D$ of bounded values can be extended to the whole interval as the measure difference vanishes. In this limit it becomes valid the last passage which relies on the approximation $\ln (1-e^{s_i} \Delta t)\approx -e^{s_i} \Delta t$.

From Bayes formula one can write the posterior as
\begin{equation}\label{posterior}
    p_{\sigma}^{(n)}\left(\boldsymbol{s}^{(n)}\Big{|} D\right) = 
    \frac{p^{(n)}\left(D | \boldsymbol{s}^{(n)}\right) \, p_{\sigma}^{(n)}\left(\boldsymbol{s}^{(n)}\right)}{p_{\sigma}^{(n)}\left( D\right)} 
    = \frac{1}{Z_{\sigma, D}^{(n)}} \exp\left(-U_{\sigma}^{(n)}[\boldsymbol{s}^{(n)}] - K_D^{(n)}[\boldsymbol{s}^{(n)}]\right)
    \equiv \frac{1}{Z_{\sigma, D}^{(n)}} \exp\left(-V_{\sigma, D}^{(n)}[\boldsymbol{s}^{(n)}]\right),
\end{equation}
where the measurement potential is
\begin{equation}
    K_D^{(n)}[\boldsymbol{s}^{(n)}] \equiv  -\sum_{i \in D} s_i + \sum_{i=0}^{n} e^{s_i} \Delta t ,
\end{equation}
the marginal $p_{\sigma}^{(n)}(D)=\int d\boldsymbol{s}^{(n)}\, p^{(n)}(D | \boldsymbol{s}^{(n)})\, p_{\sigma}^{(n)}(\boldsymbol{s}^{(n)})$, and the normalization $Z_{\sigma, D}^{(n)}(D)=\int d\boldsymbol{s}^{(n)}\, \exp\left(-V_{\sigma, D}^{(n)}[\boldsymbol{s}^{(n)}]\right)$.
The first variation of $K_D^{(n)}[\boldsymbol{s}^{(n)}]$ from the path perturbation $\epsilon \boldsymbol{\phi}^{(n)}$ is calculated as
\begin{equation}\label{variation K}
    \partial_\epsilon K_D^{(n)}[\boldsymbol{s}^{(n)}+\epsilon \boldsymbol{\phi}^{(n)}] |_{\epsilon=0} = 
    -\sum_{i \in D} \phi_i + \sum_{i=0}^n \phi_i e^{s_i} \Delta t .
\end{equation}

The posterior potential $
    V_{\sigma, D}^{(n)} \equiv U_{\sigma}^{(n)}+K_D^{(n)} $ from Eq. \eqref{posterior} accounts for the prior and the conditioning on events, and in the vanishing discretization limit $n\rightarrow 0$ it converges to the formal solution of the Bayesian problem corresponding to a particular $\sigma$.
From Eq. \eqref{variation V} and Eq. \eqref{variation K}, its gradient $\boldsymbol{\nabla}^{(n)} V_{\sigma}^{(n)}$ with respect to the path vector $\boldsymbol{s}^{(n)}$ has components
\begin{equation}\label{variation U}
    \frac{\partial V_{\sigma, D}^{(n)}}{\partial s_i} = \frac{\mathbb{I}_{i= n}-\mathbb{I}_{i=0}}{2} - \frac{\Delta t}{\sigma^2} (d_t^2 s)_i^{(n)}
    -\mathbb{I}_{i \in D}  + e^{s_i} \Delta t ,
\end{equation}
where $\mathbb{I}_{i=j}$ is the Kroeneker delta.

\paragraph*{Langevin sampling of the posterior distribution.}

A standard way of sampling an infinite-dimensional distribution like the posterior $p_{\sigma}^{(n)}(\boldsymbol{s}^{(n)}|D) = \exp\left(-V_{\sigma, D}^{(n)}[\boldsymbol{s}^{(n)}]\right) / Z_{\sigma, D}^{(n)}$ in the limit $n\rightarrow \infty$ is to consider the Langevin equation \cite{parisi1980perturbation, risken1996fokker}, that means to simulate an ergodic stochastic equilibrium dynamics which gives the target Boltzmann distribution as invariant density. Let us introduce a dummy variable $u$ for the Langevin time, not to be confused with the time axis of the original Bayesian estimation problem which is here parametrized by the vector components $i$, and by $t$ in the continuous limit $n\rightarrow\infty$.
The equilibrium Langevin equation reads
\begin{equation}\label{Langevin discrete}
    d \boldsymbol{s} = - q\,\boldsymbol{\nabla}^{(n)} V_{\sigma, D}^{(n)} \, du \,+ \sqrt{2q} \,d\boldsymbol{W}^{(n)},
\end{equation}
where $q$ is the arbitrary temperature parameter, and $d\boldsymbol{W}^{(n)}$ are standard vector Brownian motion increments in $n$ dimensions \cite{risken1996fokker, karatzas1991brownian}.
By taking $q=1/\Delta t$, in the limit $n\rightarrow \infty$ the $n$-dimensional Eq. \eqref{Langevin discrete} formally converges to
\begin{equation}\label{SPDE one}
    \partial_u s_{t, u} -\eta_{t, u} = - \frac{\delta V}{\delta s_{t, u}} \, = \frac{1}{\sigma^2} \partial^2_t s_{t, u} +\frac{1}{2}(\delta_{t,T} -\delta_{t,0}) + \sum_{u\in D} \delta_{t,u}  -e^{s_t} ,
\end{equation}
that is a stochastic partial differential equation (SPDE) \cite{parisi1980perturbation,kardar2007statistical,hairer2009introduction,lord2014introduction} driven by the space-time Gaussian white noise $\eta_{t, u}$ defined by the mean $ \langle \eta_{t, u} \rangle =0$ and covariance $ \langle \eta_{t, u} \eta_{t', u'} \rangle = 2 \delta_{t,t'} \delta_{u,u'}$, and $\delta_{t,t'}$ denotes the Dirac delta function.
The second equality in Eq. \eqref{SPDE one} comes from Eq. \eqref{variation U} and the definition of functional derivative. 
Here in Eq. \eqref{SPDE one} and in the following we omitted the explicit dependence $V\equiv V_{\sigma, D}$ to avoid confusion with the space-time variables.

\paragraph*{Uncertainty on the diffusion parameter.}

In general one does not know exactly the underlying diffusion parameter $\sigma$, such uncertainty being described by a prior $p(\sigma)$.
This will impact the above calculation as the path prior probability is modified to $p(\boldsymbol{s}) = \int d\sigma \, p(\sigma) p_{\sigma}(\boldsymbol{s})$, therefore it cannot be written as a single exponential. 
The relevant quantity is the so-called Bayesian evidence $p(\sigma | D)$, as it allows to write the posterior as $p(\boldsymbol{s}|D) = \int d\sigma \, p_\sigma(\boldsymbol{s}|D) p(\sigma | D)$.
The Bayesian evidence $p(\sigma | D)$ is the estimate, based on the observed data and on our prior knowledge $p(\sigma)$, of the unknown diffusion parameter of the dynamics generator,
\begin{equation}\label{evidence Bayes}
    p(\sigma | D) =  \frac{p(\sigma)\,p(D|\sigma)}{p(D)} =  \frac{p(\sigma)}{p(D)} \int d\boldsymbol{s}\, p(D|\boldsymbol{s})\,p_\sigma(\boldsymbol{s})
    \equiv \frac{p(\sigma) \, (\Delta t)^{|D|} }{p(D) \widetilde{Z}^{(n)}}  \, I(\sigma) ,
\end{equation}
where the dependence on the dimension $n$ is implicit, and the integral $I(\sigma) \equiv \int d\boldsymbol{s}\, e^{-V_{\sigma, D}[\boldsymbol{s}]}$ in terms of the above defined posterior potential $V$ was defined.
In the related problem of estimating a 1D normalized density from finite samples in \cite{bialek1996field,kinney2015unification}, a Bayesian evidence integral was approached with the Laplace's approximation.
Here this means to consider the limit of a small diffusion parameter $\sigma\rightarrow 0$, so that the quadratic variation becomes the dominant term in weighting the paths.
The Laplace's approximation \cite{shun1995laplace} for an exponential integral of a smooth function $V_{\sigma, D}[\boldsymbol{s}]$ of the vector $\boldsymbol{s}$ having a unique minimum in $\boldsymbol{s^*}_\sigma$ reads
\begin{equation}
    I(\sigma) \equiv \int d\boldsymbol{s} \, e^{-V_{\sigma, D}[\boldsymbol{s}]} \approx \frac{(2\pi)^\frac{n}{2}}{\sqrt{\det \left(\frac{\partial^2 U_\sigma }{\partial s_i \partial s_j}\right)}\bigg{|}_{\boldsymbol{s^*}_\sigma}} \, \exp\left(-V_{\sigma}[\boldsymbol{s^*}_\sigma]\right) ,
\end{equation}
where the Hessian matrix is computed as
\begin{equation}
    \frac{\partial^2 U_\sigma }{\partial s_i \partial s_j} =  \mathbb{I}_{i=j} e^{s_i} \Delta t + \frac{1}{\sigma^2 \Delta t} (2\mathbb{I}_{i=j} -\mathbb{I}_{i+1=j}-\mathbb{I}_{i-1=j}) ,
\end{equation}
and it is a tridiagonal matrix whose determinant can be efficiently computed.
This approximation means to neglect the tails of the distribution by assuming higher moments to behave like in a multivariate Gaussian.
The stationary point $\boldsymbol{s^*}_\sigma$ for any value of $\sigma$ is conveniently found numerically by imposing zero noise $\eta_{t, u}=0$ in the Langevin dynamics Eq. \eqref{SPDE one}.

\section{Integration convention}

We denote functions through superscripts and subscripts, $a_x\equiv a(x)$, and adopt an Einstein-like integration convention for variables repeated in superscript and subscript, $a_x b^x\equiv \int dx\, a_x b_x$, where integration is meant over the whole $(-\infty, +\infty)$ when not specified. This applies even if the repeated variables are embedded in an expression, $a_{f(x)} b^x\equiv \int dx\, a_{f(x)} b_x$.
As an example consider
\begin{equation}
    a_{2y-z} b^{x-y} c_{z,x}\equiv \iint dx\,dy\, a_{2y-z} b_{x-y} c_{z,x},
\end{equation}
where only the dependence on the variable $z$ is left after integration over $x$ and $y$ according to the convention. 
We will often use the indexed unity $1^{x, y}$ to induce integration, like in the scalar $a_{x, y} 1^{x, y} \equiv \iint dx \,dy\, a_{x, y} $.

\section{The perturbative expansion}

Let us rewrite the formal perturbative expansion (Eq. (12) in the main text),
\begin{multline}\label{Perturbative}
    x_{t, u} = y_{t, u} - G_{t-t', u-u'} \left\{ \alpha \left[ \exp\left(x^{t',u'}\right) -1^{t',u'} -x^{t',u'} \right]  + f^{t'} \left[ \exp\left(x^{t',u'}\right) -1^{t',u'} \right]  \right \} \\
    =  y_{t, u} - G_{t-t', u-u'} \bigg\{ \alpha \left[ \exp\left(y^{t',u'} - G^{t'-t'', u'-u''}  \left\{  ... \right\} \right) -1^{t',u'} -y^{t',u'} +G^{t'-t'', u'-u''}  \left\{  ... \right\} \right]  \\+ f^{t'} \left[ \exp\left(y^{t',u'} -G^{t'-t'', u'-u''}  \left\{  ... \right\} \right) -1^{t',u'} \right]  \bigg\} ,
\end{multline}
which is an implicit solution of the stochastic evolution $\partial_u x_{t, u} -\eta_{t, u} = \frac{1}{\sigma^2} \partial^2_t x_{t, u} -e^{s^*_t} (e^{x_{t, u}} -1)$ with respect to the propagator
\begin{equation}\label{G}
    G_{t, u} = \frac{\sigma \mathbb{I}_{u\geq 0}}{2\sqrt{\pi u}} \exp \left( -\alpha u -\frac{\sigma^2 t^2}{4 u} \right).
\end{equation}
This Green function corresponds to the linearized dynamics with constant coefficient $\alpha$ centered at $t=0$, and we have defined the maximum likelihood (ML) path difference accordingly as $f_t \equiv \exp[s^*_t]-\exp[s^*_0]$.
The first term $y_{t, u} \equiv G_{t-t', u-u'} \eta^{t', u'}$ in Eq. \eqref{Perturbative} is the integration of the space-time noise, the term multiplying $\alpha$ accounts for the exponential nonlinearity of the potential, and the term multiplying $f_t$ is the explicit ML path impact on the dynamics. The ML path impact on the steady-state marginal probability distribution $p(x_{0, u})$ is here studied in a perturbative expansion, that means to study its leading corrections around the space-homogeneous and Gaussian solution obtained for $f_t = 0$ and $\sigma / \sqrt{\alpha} \rightarrow 0$.
The perturbative expansion Eq. \eqref{Perturbative} allows to account for the nonlinearities and path corrections in terms of Green functions convolutions and of the multivariate Gaussian variable $y$ properties. In particular, after a Taylor expansion of the exponential nonlinearity $\exp(y) = 1+y+y^2/2 +...$, the Gaussian moments $\langle y_{t, u} y_{t', u'} y_{t'', u''} ... \rangle$ are given by the Isserlis theorem. For more background on perturbative expansions please see Refs. \cite{parisi1980perturbation, hohenberg1977theory, tauber2014critical}.

\section{Derivation of Eq. (10)}

Let us start by reviewing the well-known case of a space-homogeneous dynamics by setting $f_t=0$.
Expanding Eq. \eqref{Perturbative} up to $\mathcal{O}(y^3)$ terms we get
\begin{multline}\label{tilde Perturbative}
    \widetilde{x}_{0, 0} \equiv  x_{0, 0}\big{|}_{f_t=0} = y_{0, 0} -\alpha G_{-t, -u} \left[ \exp\left( \widetilde{x}^{t, u} \right) -1^{t, u} -\widetilde{x}^{t, u}  \right] \\
    = y_{0, 0} -\frac{\alpha}{2} G_{-t, -u} \left[ \left( y^{t, u} \right)^2 -\alpha G^{t-t', u-u'} y^2_{t', u'} y^{t, u} +\frac{1}{3} \left( y^{t, u} \right)^3 \right]  + \mathcal{O}(y^4)\\
    = y_{0, 0} -\frac{\alpha}{2} G^{-t, -u} \left[ y_{t, u}^2 -\alpha G^{t-t', u-u'} y^2_{t', u'} y_{t, u} +\frac{1}{3} y_{t, u}^3 \right]  + \mathcal{O}(y^4) . 
\end{multline}
The square is, up to $\mathcal{O}(y^4)$,
\begin{equation}\label{x2_tilde}
    \widetilde{x}_{0, 0}^2 = y_{0, 0}^2 + \frac{\alpha^2}{4} G^{-t, -u} G^{-t', -u'}  y_{t, u}^2 y_{t', u'}^2
    -\alpha G^{-t, -u}  \left[ y_{t, u}^2 -\alpha G^{t-t', u-u'} y^2_{t', u'} y_{t, u} +\frac{1}{3} y_{t, u}^3 \right] y_{0, 0} + \mathcal{O}(y^5) .
\end{equation}
The expectations of Gaussian products are computed with Isserlis theorem. For odd powers they equal zero, while for the even powers in Eq. \eqref{x2_tilde} these expectations are
\begin{equation}\label{Isserlis_1}
    \left\langle y_{t, u}^2 y_{t', u'}^2 \right\rangle = \left\langle y_{t, u}^2  \right\rangle \left\langle y_{t', u'}^2 \right\rangle + 2 \left\langle  y_{t, u}  y_{t', u'} \right\rangle^2 
    = \langle y^2 \rangle^2 1_{t,u,t',u'} +2 C_{t-t', u-u'}^2 ,
\end{equation}
\begin{equation}\label{Isserlis_2}
    \left\langle y_{0, 0} y_{t, u}  y_{t', u'} ^2 \right\rangle = \left\langle y_{0, 0} y_{t, u} \right\rangle \left\langle  y_{t', u'} ^2 \right\rangle + 2 \left\langle y_{0,0} y_{t', u'}   \right\rangle \left\langle y_{t, u} y_{t', u'}   \right\rangle
    = \langle y^2 \rangle C_{t, u} 1_{t',u'} +2 C_{t', u'} C_{t-t', u-u'},    
\end{equation}
\begin{equation}\label{Isserlis_3}
    \left\langle y_{0, 0} y_{t, u}^3 \right\rangle = 3\left\langle y_{0, 0} y_{t, u} \right\rangle \left\langle  y_{t, u} ^2 \right\rangle
    = 3 \langle y^2 \rangle C_{t, u},    
\end{equation}
where the correlation is (Eq. (10) of the main text),
\begin{equation}
    C_{t,u}\equiv \langle y_{h,q}y_{h+t, q+u} \rangle = 2G^{-t', -u'} G_{t-t', u-u'}
    = \frac{\sigma}{2\pi} \int dk \, \frac{\cos(k \sigma t) }{\alpha +k^2} e^{ -(\alpha+k^2) \,\vert u \vert },
\end{equation}
from which we find the reference Gaussian variance $\langle y^2 \rangle \equiv \langle y_{t, u}^2 \rangle = \langle y_{0, 0}^2 \rangle  = \sigma/(2\sqrt{\alpha})$.
Taking the expectation of Eq. \eqref{x2_tilde} we then obtain
\begin{multline}
    \left\langle \widetilde{x}^2 \right\rangle - \langle y^2 \rangle = \frac{1}{4} \langle y^2 \rangle^2 + \frac{\alpha^2}{2} G^{-t, -u} G^{-t', -u'}  C_{t-t', u-u'}^2 
    +2 \alpha^2 G^{-t, -u} G^{t-t', u-u'}  C_{t', u'} C_{t-t', u-u'}
    + \mathcal{O}\left(\langle y^2 \rangle^3\right) \\
    = \left( \frac{1}{4} + \frac{1}{9} \right) \langle y^2 \rangle^2
    + \mathcal{O}\left(\langle y^2 \rangle^3\right),
\end{multline}
where we used the identity $\alpha G^{t, u} 1_{t, u} = 1$, and in the last line computed the integrals using the Wolfram Mathematica software \cite{wolfram2003mathematica}. The corresponding scripts are made available in the below Github repository:\\ \textit{github.com/AndreaAuconi/BayesianFieldTheory}.

In order to give a cleaner input to the Wolfram engine we extract the dimensional factor $\langle y^2 \rangle^2$ with the transformations $k' = k/\sqrt{\alpha}$, $u' = u \alpha$, and $t' = t \sigma\sqrt{\alpha}$. The two integrals become respectively
\begin{multline}
    \frac{\alpha^2}{2} G^{-t, -u} G^{-t', -u'}  C_{t-t', u-u'}^2 = \langle y^2 \rangle^2 \frac{1}{8 \pi^3} \iint \frac{dk\,dk'}{(1+k^2)(1+{k'}^2)} \iint_{-\infty}^0 \frac{du \, du'}{\sqrt{u u'}} \times \\
     \exp \left[ u + u' -2 |u-u'| -(k^2 +{k'}^2)|u-u'| \right] \iint dt \,dt'\, \cos \left[ k (t-t') \right]  \cos \left[ k' (t-t') \right]  \exp \left[ \frac{1}{4} \left( \frac{t^2}{u} +\frac{{t'}^2}{u'}  \right) \right], 
\end{multline}
which is evaluated except for the $dk$ integral with the Wolfram script \textit{GGC2.m}, and
\begin{multline}
    2 \alpha^2 G^{-t, -u} G^{t-t', u-u'}  C_{t', u'} C_{t-t', u-u'} = \langle y^2 \rangle^2 \frac{1}{2 \pi^3} \iint \frac{dk\,dk'}{(1+k^2)(1+{k'}^2)} \int_{-\infty}^0\int_{-\infty}^u \frac{du \, du'}{\sqrt{u (u'-u)}} \times \\
    \exp \left[ -u + 3 u' +k^2 u' -{k'}^2 (u-u') \right]  \iint dt \,dt'\, \cos \left[ k t' \right]  \cos \left[ k' (t-t') \right]  \exp \left[ \frac{1}{4} \left( \frac{t^2}{u} +\frac{(t-t')^2}{u'-u}  \right) \right].
\end{multline}
which is evaluated except for the $dk$ integral with the Wolfram script \textit{GGCC.m}.
The two resulting $dk$ integrands are then summed before being integrated with the Wolfram script \textit{NonlinearityCorrection.m}, and it gives the nonlinearity correction $\langle y^2 \rangle^2 /9$, which is Eq. (13) in the main text.

\section{Other moments from the fluctuation theorem}

Let us take the expectation of Eq. \eqref{tilde Perturbative},
\begin{equation}
    \langle \widetilde{x}_{0, 0} \rangle = -\alpha G_{-t, -u} \left[ \left\langle \exp\left( \widetilde{x}^{t, u} \right) \right\rangle -1^{t, u} - \left \langle \widetilde{x}^{t, u} \right\rangle  \right]
    = -\alpha G_{-t, -u} 1^{t, u} \left[ \left\langle \exp\left( \widetilde{x}_{0, 0} \right) \right\rangle -1 - \left \langle \widetilde{x}_{0, 0} \right\rangle  \right] 
    = -\left\langle \exp\left( \widetilde{x}_{0, 0} \right) \right\rangle +1 + \left \langle \widetilde{x}_{0, 0} \right\rangle,
\end{equation}
where we used the space and time homogeneity of expectations, $p(\widetilde{x}_{t, u}) = p(\widetilde{x}_{0, 0})$.
This gives the fluctuation theorem
\begin{equation}\label{fluctuation theorem}
    1 = \left\langle \exp\left( \widetilde{x} \right) \right\rangle = \left\langle \widetilde{x} \right\rangle  +\frac{1}{2}\left\langle \widetilde{x}^2 \right\rangle + \frac{1}{6}\left\langle \widetilde{x}^3 \right\rangle +\frac{1}{24}\left\langle \widetilde{x}^4 \right\rangle 
    +\mathcal{O}\left(\langle y^2 \rangle^3\right),
\end{equation}
which we use to compute the expectation $\left\langle \widetilde{x} \right\rangle \equiv \left\langle \widetilde{x}_{0, 0} \right\rangle$ from the higher moments.

Consider the third moment,
\begin{multline}
    \left\langle \widetilde{x}^3  \right\rangle = -\frac{3}{2} \alpha G^{-t, -u} \left\langle y_{0, 0}^2 y_{t, u}^2 \right\rangle + \mathcal{O}\left(\langle y^2 \rangle^3\right)
     = -\frac{3}{2} \alpha G^{-t, -u} \left( \left\langle y_{0, 0}^2 \right\rangle \left\langle y_{t, u}^2 \right\rangle +2 \left\langle y_{0, 0} y_{t, u} \right\rangle^2 \right) + \mathcal{O}\left(\langle y^2 \rangle^3\right) \\
     = -\frac{3}{2} \alpha G^{-t, -u} \left( \langle y^2 \rangle^2 1_{t, u} +2 C_{t, u}^2 \right) + \mathcal{O}\left(\langle y^2 \rangle^3\right)
     = -\frac{3}{2} \langle y^2 \rangle^2 - 3 \alpha G^{-t, -u} C_{t, u}^2  + \mathcal{O}\left(\langle y^2 \rangle^3\right) 
      = -\frac{11}{6} \langle y^2 \rangle^2  + \mathcal{O}\left(\langle y^2 \rangle^3\right) ,
\end{multline}
where the integral
\begin{multline}
    \alpha G^{-t, -u} C_{t, u}^2
    = \langle y^2 \rangle^2 \frac{1}{2 \pi^{\frac{5}{2}}} \iint \frac{dk\,dk'}{(1+k^2)(1+{k'}^2)} \int_{-\infty}^0 \frac{du}{\sqrt{-u}}
    \exp \left[ u \left( 3 + k^2 + {k'}^2\right) \right]  \int dt \, \cos (k t) \cos (k' t)  \exp \left(\frac{t^2}{4u}  \right) \\
    = \frac{1}{9} \langle y^2 \rangle^2,
\end{multline}
was evaluated with the Wolfram script \textit{GC2.m}.
The fourth moment is $\left\langle \widetilde{x}^4  \right\rangle = \left\langle y^4  \right\rangle + \mathcal{O}\left(\langle y^2 \rangle^3\right) = 3\left\langle y^2  \right\rangle^2 + \mathcal{O}\left(\langle y^2 \rangle^3\right)$, which is already at order $\left\langle \widetilde{x}^4  \right\rangle =  \mathcal{O}\left(\langle y^2 \rangle^2\right)$, and higher order moments are negligible at this order.

From Eq. \eqref{fluctuation theorem} using the computed moments we find the expectation correction
\begin{equation}\label{tilde mu}
    \left\langle \widetilde{x}  \right\rangle = -\frac{1}{2} \langle y^2 \rangle + \mathcal{O}\left(\langle y^2 \rangle^3\right) .
\end{equation}
Then the variance correction is
\begin{equation}\label{tilde nu}
    \left\langle \widetilde{x}^2  \right\rangle - \left\langle \widetilde{x}  \right\rangle^2 -\langle y^2 \rangle = \frac{1}{9} \langle y^2 \rangle^2 + \mathcal{O}\left(\langle y^2 \rangle^3\right) ,
\end{equation}
and the skewness correction is
\begin{equation}\label{tilde skew}
    \left\langle \widetilde{x}^3  \right\rangle -3 \left\langle \widetilde{x}^2  \right\rangle \left\langle \widetilde{x}  \right\rangle +2 \left\langle \widetilde{x}  \right\rangle^3
    = -\frac{1}{3} \langle y^2 \rangle^2 + \mathcal{O}\left(\langle y^2 \rangle^3\right) .
\end{equation}

\section{The Gram–Charlier series}

We provide a visual representation of the moments corrections in terms of a truncated Gram–Charlier series, which is reviewed here in our simple setting for the reader's convenience. 
In the above expansion summarized in Eqs. \eqref{tilde mu}-\eqref{tilde skew}, we find that the marginal posterior distribution $p(\widetilde{x})$ for the homogeneous $f_t =0$ case is characterized, up to $\mathcal{O}(\langle y^2 \rangle^2)$ corrections from the Gaussian reference case, by the first three moments $\equiv \left\langle \widetilde{x}  \right\rangle$, $\left\langle \widetilde{x}^2  \right\rangle $, and $\left\langle \widetilde{x}^3  \right\rangle$.
The same structure will hold also for the spatial-dependent case discussed in the next sections, so we remove already the tilde attribute $\widetilde{x}$ to keep this section more general.

Let us write the probability density function approximation corresponding to the first three moments as a polynomial factor multiplying the Gaussian distribution $\mathcal{G}_{\mu, \xi}(x) \equiv (2\pi \xi)^{-\frac{1}{2}} \exp [-(x-\mu)^2 /(2\xi)]$ with matching mean $\mu$ and variance $\xi$,
\begin{equation}
    p(x) = \mathcal{G}_{\mu, \xi}(x) \left[ 1 + k_0 +k_1 (x-\mu) +k_2 (x-\mu)^2 +k_3 (x-\mu)^3 \right],
\end{equation}
where the truncation at four parameters reflects the number of conditions available to fit them, namely normalization, mean, variance, and skewness.
Let us denote the skewness coefficient as $\gamma \equiv \xi^{-\frac{3}{2}} \langle (x-\mu)^3  \rangle$.
The parameter fit is immediately performed as
\begin{equation}
\left\{
\begin{aligned}
& 1 = \langle 1 \rangle = 1+k_0 +k_2 \xi, \\
& 0 = \langle x-\mu\rangle = \xi (k_1 +k_3 3\xi) ,\\
& \xi = \langle (x-\mu)^2 \rangle = \xi (1 +k_0 + k_2 3 \xi), \\
& \gamma \xi^{\frac{3}{2}} = \langle (x-\mu)^3 \rangle = 3 \xi^2 (k_1 +k_3 5 \xi) ,
\end{aligned}
\right.
\implies
\left\{
\begin{aligned}
& k_0 = k_2 = 0, \\
& k_3 = \frac{\gamma}{6} \xi^{-\frac{3}{2}}, \\
& k_1 = -3 k_3 \xi,
\end{aligned}
\right.
\end{equation}
where we used the Gaussian properties $\int dx\, \mathcal{G}_{\mu, \xi}(x)\, (x-\mu)^4 = 3 \xi^2$ and $\int dx\, \mathcal{G}_{\mu, \xi}(x)\, (x-\mu)^6 = 5\cdot 3 \xi^3$.
The approximated density is then
\begin{equation}\label{Gram–Charlier}
    p(x) = \mathcal{G}_{\mu, \xi}(x) \left\{ 1 + \frac{\gamma}{6} \left[ \left(\frac{x-\mu}{\sqrt{\xi}}\right)^3 -3\left(\frac{x-\mu}{\sqrt{\xi}}\right) \right] \right\}.
\end{equation}
This representation of Eq. \eqref{Gram–Charlier} is not a probability distribution function because it is negative for values $x-\mu < - \sqrt{\xi} \left(6/\gamma \right)^{1/3}$, but it is an approximation valid in the region where $x-\mu = \mathcal{O}(\sqrt{\xi})$. Indeed, from Eq. \eqref{tilde skew} we see that $\gamma = -\frac{1}{3}\sqrt{\xi} +\mathcal{O(\xi \sqrt{\xi})} = \mathcal{O}(\sqrt{\xi})$, and on the relevant scale where $x-\mu = \mathcal{O}(\sqrt{\xi})$ the correction becomes small in the limit $\xi\rightarrow 0$.

\section{Perturbative order of path corrections}

Before approaching the perturbative expansion for evaluating the ML path corrections, we need to show that the ML path fluctuations $f_t \equiv \exp[s^*_t]-\exp[s^*_0]$ are statistically large enough for their impact on the moments to appear at or before the order $\mathcal{O}(\langle y^2 \rangle^2)$ we considered above. 

Let us start writing explicitly Eq. (5) of the main text, that is the equation characterizing the ML dynamics, $(\delta V/\delta s_t) \big|_{\boldsymbol{s}^*} = 0$. For $0<t<T$ this reads
\begin{equation}\label{ML second order}
       d^2_t s^*_t
        = \sigma^2 \left( e^{s^*_t} - \sum_{u\in D} \delta_{t,u} \right) .
\end{equation}

Consider the true rate dynamics $dr = \sigma r dW$, which is a driftless GBM whose formal solution in terms of the noise realization is $\ln \left( r_t/r_0 \right) = \sigma W_t -\sigma^2 t/2$.
In the small fluctuations limit $\langle y^2 \rangle \ll 1$ we see that the dynamics on the correlation timescale $\tau=1/(\sigma\sqrt{\alpha})$ is in the diffusive phase where statistically $|W_\tau|\gg \sigma \tau$.
Then the log-rate variation on the correlation timescale is of order $\ln \left( r_\tau/r_0 \right) = \mathcal{O}\left( \sigma \sqrt{\tau} \right)  = \mathcal{O}\left( \sqrt{\langle y^2 \rangle} \right)$, which vanishes in the limit $\langle y^2 \rangle \rightarrow 0 $.
The discrepancy between the ML log-path $s^*_t$ from the true log-rate $s_t=\ln r_t$ is of order $s^*_t -s_t = \mathcal{O}(\sqrt{\langle y^2 \rangle})$, therefore the ML log-path displacement is also vanishing in the small fluctuations limit as $s^*_t -s^*_0 = \ln \left( r_\tau/r_0 \right) + \mathcal{O}(\sqrt{\langle y^2 \rangle}) = \mathcal{O}(\sqrt{\langle y^2 \rangle})$.
Then we can study the ML path fluctuations $f_t \equiv \exp[s^*_t]-\exp[s^*_0]$ in this limit by linerization of
\begin{equation}
    s^*_t \equiv \ln(h_t) \approx \ln (h_0) + \frac{h_t-h_0}{h_0} = \ln(\alpha) + \frac{h_t}{\alpha} -1 .
\end{equation}
The ML path defining Eq. \eqref{ML second order} in terms of $h_t$ reads
\begin{equation}
          d^2_t h_t
        = \alpha\sigma^2 \left( h_t - \sum_{u\in D} \delta_{t,u} \right) .
\end{equation}
This equation is satisfied by the Kalman smoother \cite{petris2009dynamic},
\begin{equation}\label{Kalman smoother}
    h_t = \frac{\sigma\sqrt{\alpha}}{2} \sum_{u\in D} \exp\left( -\sigma\sqrt{\alpha} |t-u| \right) ,
\end{equation}
which integrates the set of events $u\in D$ with an exponential kernel of timescale $\tau=1/(\sigma\sqrt{\alpha})$ equal to the correlation timescale. Note that $\alpha\equiv \exp (s^*_0)$ is not known a priori but it is a result of the maximum likelihood path calibration.
The time derivative of the smoother is
\begin{equation}
    d_t h_t = -\frac{\sigma^2 \alpha}{2} \sum_{u\in D} \operatorname{sgn}(t-u) \exp\left( -\sigma\sqrt{\alpha} |t-u| \right) ,
\end{equation}
and it is almost surely finite except for the finite discontinuities at the events' time instants $u\in D$.
Let us consider expectations $\mathbb{E}$ with respect to the true GBM $r_t$ and events realizations $u\in D$. We take for simplicity the condition, not known by the estimator, that $r_0$ is fixed.
The GBM is not reversible in time, as indeed the evolution increases the log-normal skewness, and the corresponding log-process $s_t$ has an explicit drift $ds = \sigma dW -\sigma^2 dt/2$. The backward log-process $s^{(B)}_t\equiv s_{-t}$ is then described by the evolution $ds^{(B)}_t = \sigma dW +\sigma^2 dt/2$, which for the backward rate gives $r_t^{(B)} = r_0 \exp\left(\sigma W_t +\sigma^2 t/2 \right)$.
Accordingly, let us write the conditional expectation at $t=0$ as
\begin{multline}\label{E events exp}
   \mathbb{E} \left[ \sum_{u\in D} e^{-\sigma\sqrt{\alpha} |u|} \bigg{|} r_0 \right] = \int dt' \,\mathbb{E}\left[ r_{t'} \big{|} r_0 \right] e^{-\sigma\sqrt{\alpha} |t'|} 
   = r_0 \int dt' \, \left[ \mathbb{I}_{t'\geq 0} + \mathbb{I}_{t' < 0} e^{-\sigma^2 t'} \right] e^{-\sigma\sqrt{\alpha} |t'|} \\
  = \frac{r_0}{\sigma\sqrt{\alpha}} \left( 1 + \frac{1}{1-\sigma/\sqrt{\alpha}} \right) = \frac{2 r_0}{\sigma\sqrt{\alpha}} \left[1 + \langle y^2 \rangle +\mathcal{O}\left(\langle y^2 \rangle^2\right)\right],
\end{multline}
where again we are considering the small fluctuations limit $\sigma \ll \sqrt{\alpha}$. Note that we are integrating over the real line neglecting border effects while in the numerical experiments we practically consider a finite region of time length "much" larger than the correlation time, $T=10\,\tau \gg \tau$, and shift it by $-T/2$ to be centered in $t=0$.
From Eq. \eqref{E events exp} we find that the expectation of the Kalman smoother is unbiased at leading order,
\begin{equation}
    \mathbb{E}\left[ h_0 | r_0 \right] = r_0 \left( 1+ \langle y^2 \rangle \right) + \mathcal{O}(r_0 \langle y^2 \rangle^2).
\end{equation}

In the small fluctuations limit, the probability density of two time instants $t'$ and $t''$ corresponding to events is
\begin{equation}
    p\left(t'\in D,\, t'' \in D \,\big{|} r_0\right) 
    = \delta_{t', t''} \mathbb{E}\left[ r_{t'} | r_0 \right]  + \mathbb{E}\left[ r_{t'} r_{t''} | r_0 \right] ,
\end{equation}
where $\delta_{t', t''}$ denotes the Dirac delta function.
The conditional covariance terms are computed as
\begin{equation}
    \mathbb{E}\left[ r_{t'} r_{t''} | r_0 \right] = r_0^2 \left(\mathbb{I}_{t'\geq 0, t''<0} \,e^{-\sigma^2 t''} +\mathbb{I}_{t'< 0, t''\geq 0}\, e^{-\sigma^2 t'}
    +\mathbb{I}_{t'\geq 0, t''\geq 0}\, e^{\sigma^2 \min (t', t'')} +\mathbb{I}_{t'< 0, t''< 0}\, e^{-\sigma^2 \left( t' + t'' + \max (t', t'') \right)} \right),
\end{equation}
where the last term was evaluated from the backward process for positive times with $t''\geq t' >0$ as
\begin{equation}\label{underlying covariance}
     \mathbb{E}\left[ r^{(B)}_{t'} r^{(B)}_{t''} \big{|} r^{(B)}_{0} \right] =
     \mathbb{E}\left[ r^{(B)}_{t'}  \mathbb{E}\left[ r^{(B)}_{t''} \big{|} r^{(B)}_{t'} \right] \big{|} r^{(B)}_{0} \right]
     = e^{\sigma^2 (t''-t')} \,\mathbb{E}\left[ \left(r^{(B)}_{t'}\right)^2 \big{|} r^{(B)}_{0} \right] = e^{\sigma^2 (2t'+t'')} = e^{\sigma^2 (t'+t''+\min (t', t''))} .
\end{equation}

The second moment of the Kalman smoother is evaluated with the Wolfram script \textit{q2.m} as
\begin{multline}
    \mathbb{E}\left[ h_0^2 | r_0 \right] = \frac{\sigma^2 \alpha}{4}\int\int dt' dt'' \, e^{-\sigma\sqrt{\alpha} (|t'| +|t''|)} \, p\left(t'\in D,\, t'' \in D \,\big{|} r_0\right) \\
    = r_0\alpha \frac{1}{8} \frac{4\sigma/\sqrt{\alpha}-(\sigma/\sqrt{\alpha})^2}{2-\sigma/\sqrt{\alpha}}
    + r_0^2 \frac{4-3\sigma/\sqrt{\alpha}}{4-8\sigma/\sqrt{\alpha}+3(\sigma/\sqrt{\alpha})^2}
    =r_0^2 \left(1+\frac{5}{2}\langle y^2\rangle\right) +r_0 \frac{\alpha}{2}\langle y^2\rangle
    +\mathcal{O}\left(\alpha^2\langle y^2 \rangle^2 \right),
\end{multline}
and note that to leading order $r_0\approx\alpha$. Then the variance is
\begin{equation}
    \mathbb{E}\left[ h_0^2 | r_0 \right] -\left(\mathbb{E}\left[ h_0 | r_0 \right]\right)^2 = r_0 \langle y^2\rangle \frac{1}{2} (r_0 +\alpha) +\mathcal{O}\left(\alpha^2\langle y^2 \rangle^2 \right) = r_0^2 \langle y^2\rangle +\mathcal{O}\left(\alpha^2\langle y^2 \rangle^2 \right)  ,
\end{equation}
and it is consistent with the posterior rate variance,
\begin{equation}
   \left\langle \left( e^{s_0} -e^{s^*_0}\right)^2 \right\rangle
   = e^{2s^*_0} \left\langle \left( e^{s_0-s^*_0} -1\right)^2 \right\rangle
   = \alpha^2 \left\langle \left(e^{x_{0, 0}} -1 \right)^2 \right\rangle
   \approx \alpha^2\langle y^2 \rangle
   \approx r_0^2 \langle y^2 \rangle\big{|}_{\alpha=r_0}, 
\end{equation}
which verifies that the full Bayesian problem converges to the Kalman smoother in the limit of small fluctuations $\langle y^2 \rangle\rightarrow 0$.

The Kalman smoother expected velocity is of order $\mathbb{E}\left[ (d_t h_t)_0 | r_0 \right] = \mathcal{O}(r_0 \sigma \sqrt{\alpha} \langle y^2 \rangle)$, which on the correlation timescale $\tau = 1/(\sigma\sqrt{\alpha})$ is statistically negligible compared to the diffusive scaling $r_t-r_0 = \mathcal{O} (r_0 \sigma \sqrt{\tau})$,
\begin{equation}
    \frac{\left(\mathbb{E}\left[ (d_t h_t |_0) | r_0 \right]\right)^2 \tau^2}{ \mathbb{E}\left[(r_\tau - r_0)^2 | r_0 \right]}  = \mathcal{O}\left(\langle y^2 \rangle \right) .
\end{equation}
Nevertheless, the fluctuations of the velocity $(d_t h_t)_0$ are evaluated with the Wolfram script \textit{scaling.m} as
\begin{multline}
    \mathbb{E}\left[ (d_t h_t)^2_0 | r_0 \right] = \frac{\sigma^4 \alpha^2}{4}\int\int dt' dt'' \, \operatorname{sgn}(t')  \operatorname{sgn}(t'')\, e^{-\sigma\sqrt{\alpha} (|t'| +|t''|)} \, p\left(t'\in D,\, t'' \in D \,\big{|} r_0\right) \\
    = \frac{1}{4}r_0 \sigma^3 \sqrt{\alpha}  \left( r_0 + \alpha\right) \left( 1+\mathcal{O}(\langle y^2 \rangle) \right)
    \approx \frac{1}{2} \sigma^3 \alpha^{5/2},
\end{multline}
where we considered only leading order terms in the limit $\langle y^2 \rangle\rightarrow 0$, and accordingly approximated $\alpha\equiv e^{s^*_0}\approx r_0$.
Then, comparing the mean squared displacement of the Kalman smoother to that of the underlying diffusive process, both evaluated at the correlation timescale,
\begin{equation}\label{1/2 scaling}
   \frac{\mathbb{E}\left[ f_\tau^2 | r_0 \right]}{ \mathbb{E}\left[(r_\tau - r_0)^2 | r_0 \right]}
   \approx \frac{\mathbb{E}\left[ (d_t h_t|_0)^2 | r_0 \right] \tau^2}{ \mathbb{E}\left[(r_\tau - r_0)^2 | r_0 \right]}  \approx \frac{1}{2},
\end{equation}
we find that they have asymptotically the same order.

Let us discuss the implications of this result to our perturbative expansion.
The ML path $\exp(s^*_t)$ has a higher regularity than the true path $r_t$, as indeed its velocity is defined on all points except of a set of zero measure corresponding to the events $u\in D$.
This fact, however, does not mean that we can neglect the path corrections in the small fluctuations limit $\langle y^2 \rangle \rightarrow 0$. In fact, on the relevant timescale where the path corrections will be integrated, that is the correlation timescale $\tau=1/(\sigma\sqrt{\alpha})$, the ML path will have accumulated a deviation $f_t$ which is statistically of the same order of the diffusive scaling.
In other words, while on large timescales $t\gg \tau$ the ML dynamics follows the true underlying diffusive process $f_t \sim \mathcal{O}(\sqrt{t})$, and on small timescales $t\ll \tau$ the ML path is practically smooth $f_t \sim \mathcal{O}(t)$ and negligible with respect to the diffusive phase, we find that on the relevant timescale $\tau$ of Bayesian estimation the ML path is also macroscopic and cannot be neglected. We denote this fact as
\begin{equation}\label{f sim y}
    \mathcal{O}(y) \sim \mathcal{O}(f_{\tau}) , 
\end{equation}
where the order is meant in the statistical sense.
In the perturbative expansion of the ML path impact below, this result means that we will have to treat $f_t$ as the same order as $y$.
We verify this asymptotic scaling and the factor $1/2$ in Eq. \eqref{1/2 scaling} by numerical simulations in Fig. (\ref{fig:scaling}).

\begin{figure}
    \centering    \includegraphics[width=0.47\linewidth]{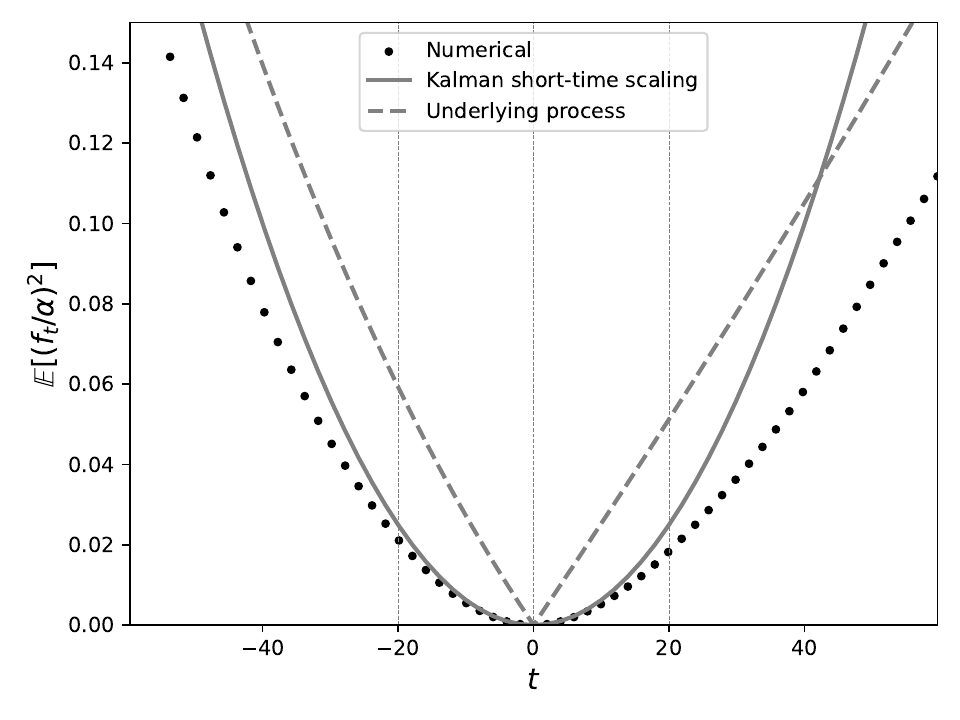}
    \includegraphics[width=0.47\linewidth]{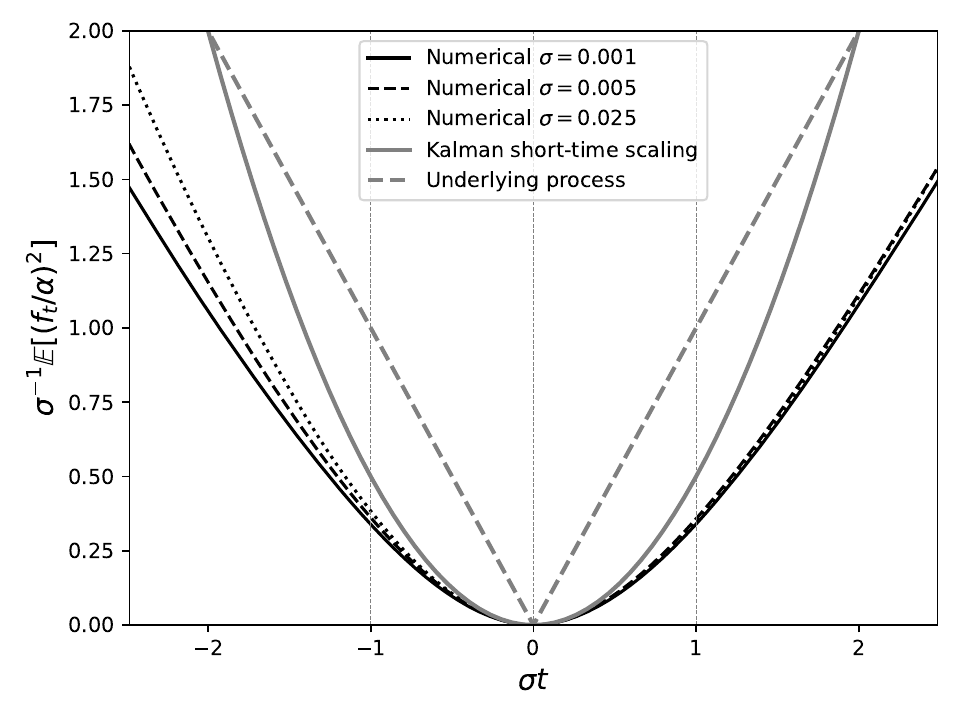}
    \caption{The mean squared displacement (msd) $\mathbb{E} \left[f_t^2 \right]$ of the maximum likelihood curve $\exp(s^*_t)\equiv \exp(s^*_0) +f_t$ is estimated by numerical integration of the PDE $\partial_u s_{t, u} =    -\delta V/\delta s_{t, u}$, see Eq. (5) of the main text, for a sufficiently long time for the dynamics to relax to the fixed point $s^*_{t}$. The dotted vertical lines are placed at $\pm \tau$ corresponding to the correlation time $\tau \equiv 1/(\sigma\sqrt{\alpha})$. A description in terms of the statistics of the instantaneous velocity of the Kalman smoother, see Eq. \eqref{Kalman smoother}, is able to capture the short-time scaling of the msd. While in the limit $t\rightarrow 0$ we see that the ML path has an higher degree of regularity $f_t\sim \mathcal{O}(t)$ compared to the underlying diffusive rate $r_t\sim \mathcal{O}(\sqrt{t})$, on the correlation timescale $t=\tau$ the mean squared displacements of the two processes are of the same order, see Eq. \eqref{1/2 scaling}. On longer timescales $t\gg \tau$ the uncertainty $\sqrt{\langle y^2 \rangle}$ is statistically much smaller than the displacement $f_t\approx r_t-r_0$ and the ML path msd behaves like that of the underlying process.
    Note that the slight time asymmetry is given by the irreversibility of the underlying GBM process from the imposed condition $r_0 = 1$.
    (Left ) Here the volatility parameter is $\sigma = 0.05$. (Right) Here we compare three different values of $\sigma$ and renormalize the coordinates to show the convergence of $\mathbb{E} \left[f_\tau^2 \right]/(\sigma^2\alpha^2 \tau)$ to a finite ratio for $\sigma\rightarrow 0$, which motivates our scaling hypothesis. Note that in the small fluctuations limit $\alpha\approx r_0 = 1$ so $\nu\approx \sigma/2$ and $\tau\approx \sigma^{-1}$. The Underlying process is here plotted in the limit $\sigma\rightarrow 0$ where $r_t\approx r_0 \sigma W_t$.
    }
    \label{fig:scaling}
\end{figure}

\section{Derivation of Eq. (14)}
Based on the asymptotic behavior summarized by Eq. \eqref{f sim y}, in this section we derive the path impacts on the variance $\langle x^2 \rangle-\langle x \rangle^2$.
Consider the perturbative expansion of the process in the approximation center $t=0$ for an arbitrary $u=0$,
\begin{equation}
    x_{0, 0} = y_{0, 0} - G_{-t, u} \left\{ \alpha \left[ \exp\left(x^{t, u}\right) -1^{t,u} -x^{t,u} \right]  + f^{t} \left[ \exp\left(x^{t,u}\right) -1^{t,u} \right]  \right \}
    = \widetilde{x}_{0, 0} +\delta x_{0, 0} + \mathcal{O}(y^4),
\end{equation}
where $\widetilde{x}_{0, 0}$ is the homogeneous drift ($f_t=0$) solution we have introduced above in Eq. \eqref{tilde Perturbative}, and the path correction is
\begin{equation}
    \delta x_{0, 0} = -G_{-t, -u} \left\{ 
    -\alpha y^{t, u} G^{t-t', u-u'}f_{t'}y_{t', u'}
    +f^t \left[ y^{t, u} -G^{t-t', u-u'} \left( \frac{\alpha}{2} y^2_{t', u'} +f_{t'}y_{t', u'} \right) 
    +\frac{1}{2} \left( y^{t, u}  \right)^2\right]
    \right\} 
    + \mathcal{O}(y^4).
\end{equation}
The squared correction is
\begin{equation}
    (\delta x_{0, 0})^2 = G_{-t, -u}G_{-t', -u'}f^t f^{t'} y^{t, u} y^{t', u'} +\mathcal{O}(y^5),
\end{equation}
and its expectation
\begin{equation}
    \left\langle(\delta x_{0, 0})^2 \right\rangle= G_{-t, -u}G_{-t', -u'} C^{t-t', u-u'} f^t f^{t'} +\mathcal{O}\left( \langle y^2\rangle^{5/2} \right),
\end{equation}
The cross term is
\begin{equation}
    \widetilde{x}_{0, 0} \,\delta x_{0, 0} = y_{0, 0} \,\delta x_{0, 0} + \frac{\alpha}{2} G^{-t, -u} y^2_{t, u} G^{-t', -u'} y_{t', u'} f_{t'} +\mathcal{O}(y^5),
\end{equation}
and its expectation
\begin{equation}
    \langle \widetilde{x}_{0, 0} \,\delta x_{0, 0} \rangle
    = -G_{-t, -u} f^t \left( C^{t, u} - G^{t-t', u-u'} f_{t'} C_{t', u'} \right) +\mathcal{O}\left( \langle y^2\rangle^{5/2} \right) .
\end{equation}
From these we can now compute the variance
\begin{multline}\label{variance path corrections}
  \left\langle x^2 \right\rangle -\langle x \rangle^2 = \langle \widetilde{x}^2 \rangle +\langle (\delta x_{0, 0})^2 \rangle +2 \langle \widetilde{x}_{0, 0} \,\delta x_{0, 0} \rangle -\langle \widetilde{x} \rangle^2 +\mathcal{O}\left( \langle y^2\rangle^{5/2} \right)
  \\ = \langle y^2 \rangle + \frac{1}{9} \langle y^2 \rangle^2 + J_t f^t  + K_{t, t'} f^t f^{t'} +\mathcal{O}\left( \langle y^2\rangle^{5/2} \right),
\end{multline}
where we defined
\begin{equation}\label{def J}
    J_t \equiv -2 G_{-t, -u} {C_{t,}}^{u},
\end{equation}
and
\begin{equation}\label{def K}
    K_{t, t'} \equiv 2 G_{-t, -u} {G_{t-t',}}^{u-u'} C_{t', u'}
    + G_{-t, -u}G_{-t', -u'} {C_{t-t',}}^{u-u'}.
\end{equation}

\section{The $J_t f^t$ leading shape correction}
The leading order path impact on the variance is given by $J_t f^t$.
Let us start by considering the kernel explicitly
\begin{multline}\label{J_t}
    J_t \equiv -2 G_{-t, -u} {C_{t,}}^{u} 
    = - \frac{\sigma^2}{2 \pi^{3/2}} \int dk \,\frac{\cos(k\sigma t)}{\alpha + k^2} \int_{-\infty}^0 \frac{du}{\sqrt{-u}}\, \exp\left[ (2\alpha +k^2) u +\frac{\sigma^2 t^2}{4 u} \right] \\
    = - \frac{\sigma^2}{2 \pi} \int dk \,\frac{\cos(k\sigma t)}{(\alpha + k^2) \sqrt{2\alpha +k^2}} \exp\left( -\sigma |t| \sqrt{2\alpha +k^2} \right) \\
    = -\langle y^2 \rangle^2 \,\frac{2}{\pi} \int dk\, \frac{\cos\left(k \frac{t}{\tau}\right)}{(1 + k^2) \sqrt{2 +k^2}} \exp\left( -\frac{|t|}{\tau} \sqrt{2 +k^2} \right),
\end{multline}
where we integrated in $du$ using the integral $\int_0^{\infty} dx\, e^{-\gamma x -\beta/x} x^{-1/2} = \sqrt{\pi/\gamma}\, e^{-2\sqrt{\beta \gamma}} $ (with $\beta>0$, $\gamma>0$) from Ref. \cite{gradshteyn2014table} (7th Ed., pg. 369), then rewrote the frequency integral in non-dimensional form with the transformation $k'=k/\sqrt{\alpha}$, and we are using the correlation time definition $\tau\equiv1/(\sigma\sqrt{\alpha})$.

If we would use the Kalman smoother in the short-time regime $f_t \approx (d_t h_t)_0 t$ corresponding to a constant velocity as used above to derive Eq. \eqref{1/2 scaling}, then the integral $J_t f^t$ would be identically zero by symmetry.
Considering a second order expansion using $d^2_t h_t$ is not possible even in an approximation given its divergence at the event times.
In principle we could evaluate the covariance of the Kalman smoother $\mathbb{E}[h_t h_{t'}]$, but this is a cumbersome integral given the many regions arising from the piecewise definitions of both $h_t$ in Eq. \eqref{Kalman smoother} and the underlying process covariance in Eq. \eqref{underlying covariance}.
We instead leverage the scaling concept of Eq. \eqref{f sim y} according to which the path impact $J_tf^t$ should statistically be of order $\mathcal{O}(\langle y^2\rangle^{3/2})$ as it contains a correlation $C\sim \mathcal{O}(y^2)$ and the path $f_\tau \sim \mathcal{O}(y)$.
In other words, in the limit of small fluctuations the path impact $J_tf^t$ will have the same scaling as $J^t (r_t-r_01_t)$, that is the same functional but evaluated at the true path $r_t$, and will differ from it only by a prefactor.

From the true path expectation conditioned on $r_0$, that is $\mathbb{E}\left[ r_{t} \big{|} r_0 \right] 
   = r_0  \left( \mathbb{I}_{t\geq 0} + \mathbb{I}_{t < 0} e^{-\sigma^2 t} \right) $, we compute the conditional expectation of the correction as
\begin{multline}
    \mathbb{E}\left[ J_t f^t \big{|} r_0 \right] \sim  \mathbb{E}\left[ J^t \left( r_t -r_0 1_t \right) \big{|} r_0 \right] 
    = r_0 \langle y^2 \rangle^2 \,\frac{2}{\pi} \int \frac{dk}{(1 + k^2) \sqrt{2 +k^2}} \int_{0}^\infty dt\, \cos\left(k \frac{t}{\tau}\right) e^{-\frac{t}{\tau} \sqrt{2 +k^2} }    \left( e^{\sigma^2 t} -1 \right) \\
    = \frac{r_0}{\alpha} \langle y^2 \rangle^2 \,\frac{1}{\pi} \int \frac{dk}{(1 + k^2)^3 \sqrt{2 +k^2}}  \,+ \mathcal{O}\left(\langle y^2 \rangle^3\right) 
    = \frac{r_0}{4\alpha} \langle y^2 \rangle^2 + \mathcal{O}\left(\langle y^2 \rangle^3\right)  = 
    \frac{1}{4} \langle y^2 \rangle^2 + \mathcal{O}\left(\langle y^2 \rangle^3\right),
\end{multline}
which means that the time irreversibility of the GBM already contributes an expected correction of the same order $\mathcal{O}\left(\langle y^2 \rangle^2\right)$ of the nonlinearity corrections.

Consider the covariance 
\begin{multline}
\mathbb{E}\left[ (r_t-r_0)(r_{t'}-r_0) | r_0\right] = r_0^2 \left[ \mathbb{I}_{t\geq 0, t'\geq 0}\, \left( e^{\sigma^2 \min (t, t')} - 1 \right) +\mathbb{I}_{t< 0, t'< 0}\, \left( e^{-\sigma^2 \left( t + t' + \max (t, t') \right)} - e^{-\sigma^2 t'} - e^{-\sigma^2 t} + 1 \right) \right]\\
\approx
\mathbb{I}_{tt'\geq 0} r_0^2 \sigma^2 \min (|t|, |t'|) ,
\end{multline}
where in the second line we have taken only the first order in the exponential functions as on the correlation timescale $\sigma\tau\ll 1$, and we joined the two cases using the absolute value and the relation $\mathbb{I}_{tt'\geq 0} = \mathbb{I}_{t\geq 0, t'\geq 0}+\mathbb{I}_{t< 0, t'< 0}$.
Then we compute
\begin{multline}\label{Jf underlying scaling}
    \mathbb{E}\left[\left(J^t (r_t-r_01_t)\right)^2 \big{|} r_0 \right] =
    J^tJ^{t'}\mathbb{E}\left[(r_t-r_01_t)(r_{t'}-r_01_{t'}) \big{|} r_0 \right]
  = 2 r_0^2 \sigma^2 J^t J^{t'} \mathbb{I}_{t\geq 0, t'\geq 0} \min (|t|, |t'|)\\
  = 4 r_0^2 \sigma^2 J^t J^{t'} \mathbb{I}_{t\geq t'\geq 0} t'\\
  = \frac{16}{\pi^2} r_0^2 \sigma^2 \langle y^2 \rangle^2 \, \iint  \frac{dk\,dk'}{(1 + k^2) \sqrt{2 +k^2} (1 + {k'}^2) \sqrt{2 +{k'}^2}} \times \\
  \times \int_0^{\infty}dt \int_0^t dt'\, t'\,\cos\left(k \frac{t}{\tau}\right) \cos\left(k' \frac{t'}{\tau}\right) \exp\left[ -\frac{1}{\tau} \left( t\sqrt{2 +k^2}+t'\sqrt{2 +{k'}^2} \right) \right] \\
  = \frac{16}{\pi^2} r_0^2 \sigma^2 \tau^3 \langle y^2 \rangle^4 \, \iint  \frac{dk\,dk'}{(1 + k^2) \sqrt{2 +k^2} (1 + {k'}^2) \sqrt{2 +{k'}^2}} \times \\
  \times \int_0^{\infty}dt \int_0^t dt'\, t'\,\cos\left(k t\right) \cos\left(k' t'\right) \exp\left[ - \left( t\sqrt{2 +k^2}+t'\sqrt{2 +{k'}^2} \right) \right] \\
  =\frac{1}{8} r_0^2 \sigma^2 \tau^3 \langle y^2 \rangle^4 = \frac{1}{16} \left(\frac{r_0}{\alpha}\right)^2 \langle y^2 \rangle^3
  \approx \frac{1}{16} \langle y^2 \rangle^3,
\end{multline}
where the non-dimensional integral was evaluated with the Wolfram script \textit{J\_correction.m}.
This scaling was verified numerically in Fig. \ref{fig:3_2_scaling}, and it is indirectly a test of the scaling logic of Eq. \eqref{f sim y} that we have already applied in the perturbative expansion to derive the path corrections of Eq. \eqref{variance path corrections}.

Applying the same scaling logic to the second order path impact $K_{t, t'} f^t f^{t'}$, this should statistically be of order $\mathcal{O}(\langle y^2 \rangle^{2})$ as it contains a correlation $C\sim \mathcal{O}(y^2)$ and a product of paths $f_\tau f_\tau \sim \mathcal{O}(y^2)$.

\begin{figure}
    \centering    \includegraphics[width=0.5\linewidth]{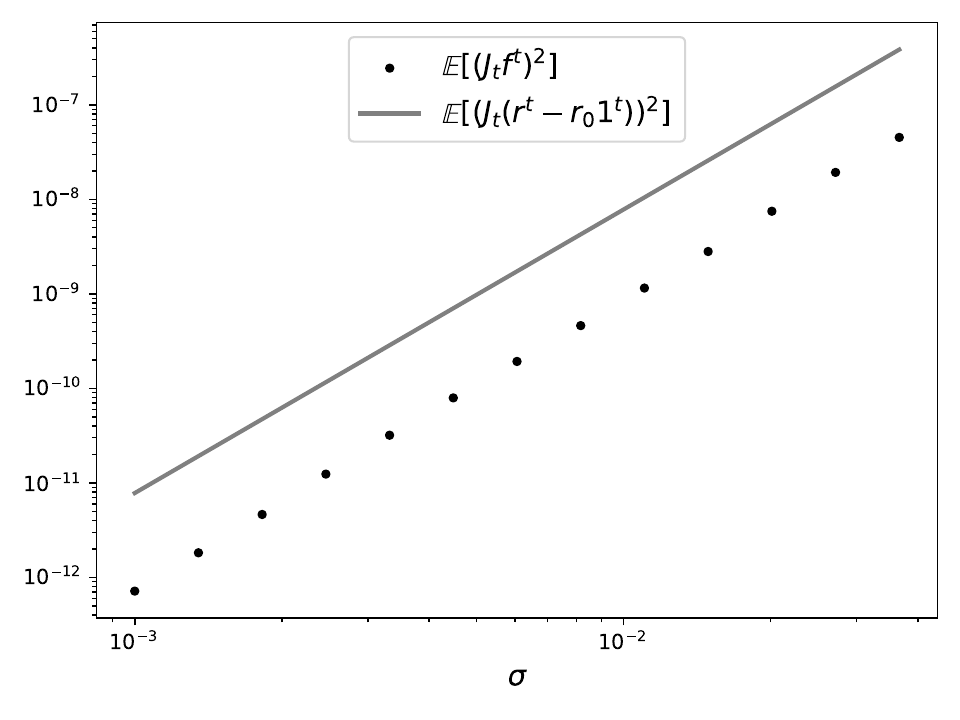}
    \caption{Numerical test of the scaling of Eq. \eqref{f sim y} through its impact on the leading path correction to the variance $J_t f^t$. In particular, the scaling $\sim \langle y^2 \rangle^3$ (here $1=r_0\approx\alpha$ so that $\langle y^2 \rangle \approx \sigma/2$) applies both to the underlying process $\mathbb{E}\left[\left(J^t (r_t-r_01_t)\right)^2 \big{|} r_0 \right]$, which was analytically computed in Eq. \eqref{Jf underlying scaling}, and also to the path correction $\mathbb{E}\left[\left(J^t f_t\right)^2 \big{|} r_0 \right]$.}
    \label{fig:3_2_scaling}
\end{figure}

\begin{figure}
    \centering    \includegraphics[width=0.32\linewidth]{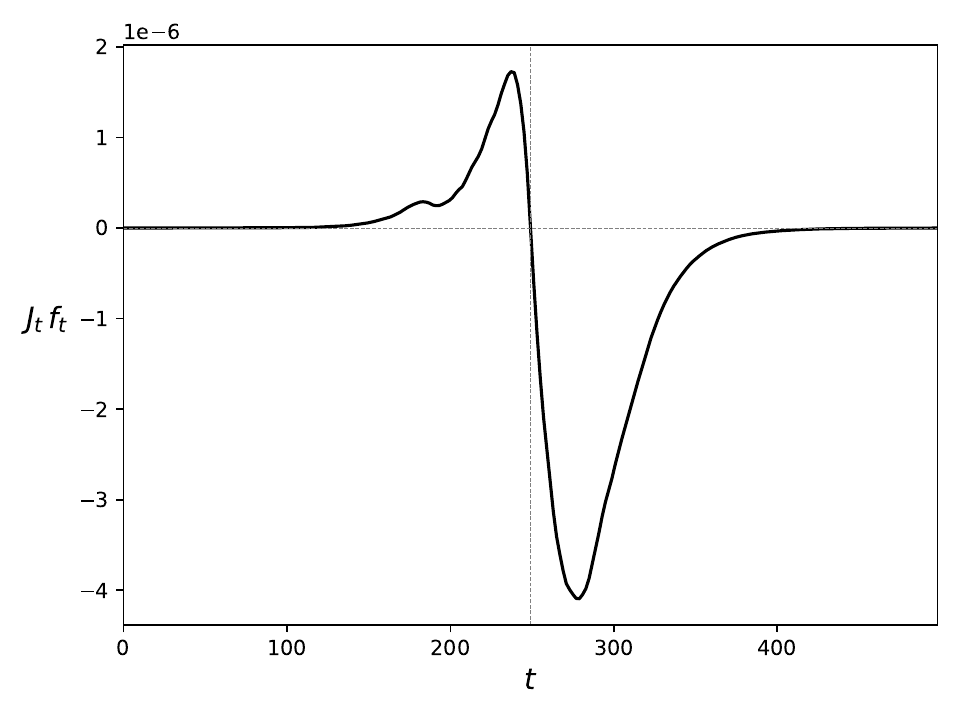}
    \includegraphics[width=0.32\linewidth]{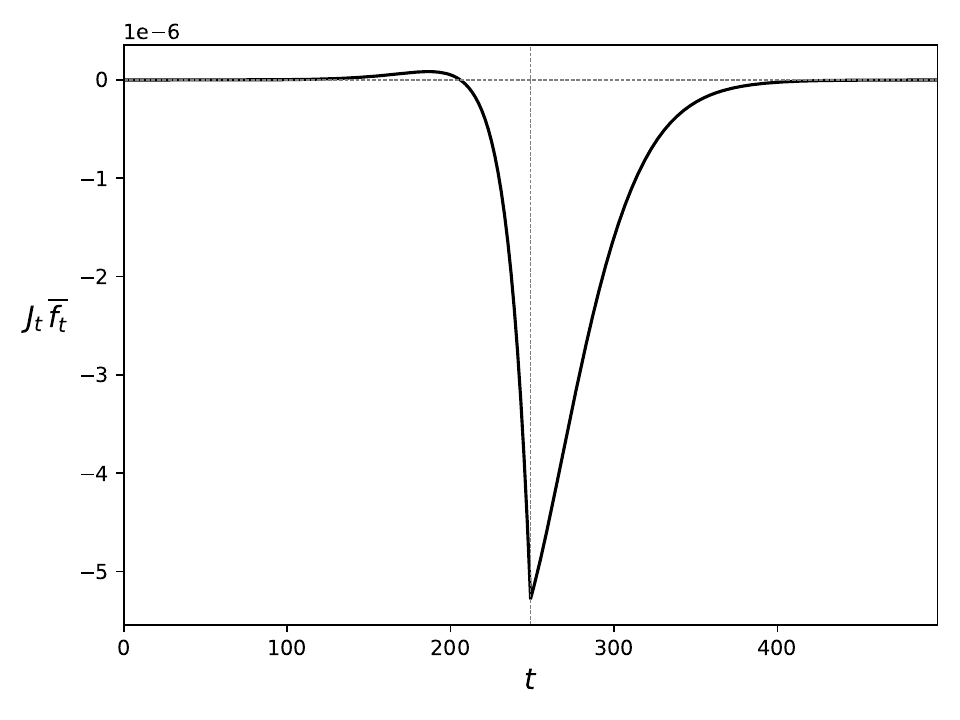}
    \includegraphics[width=0.32\linewidth]{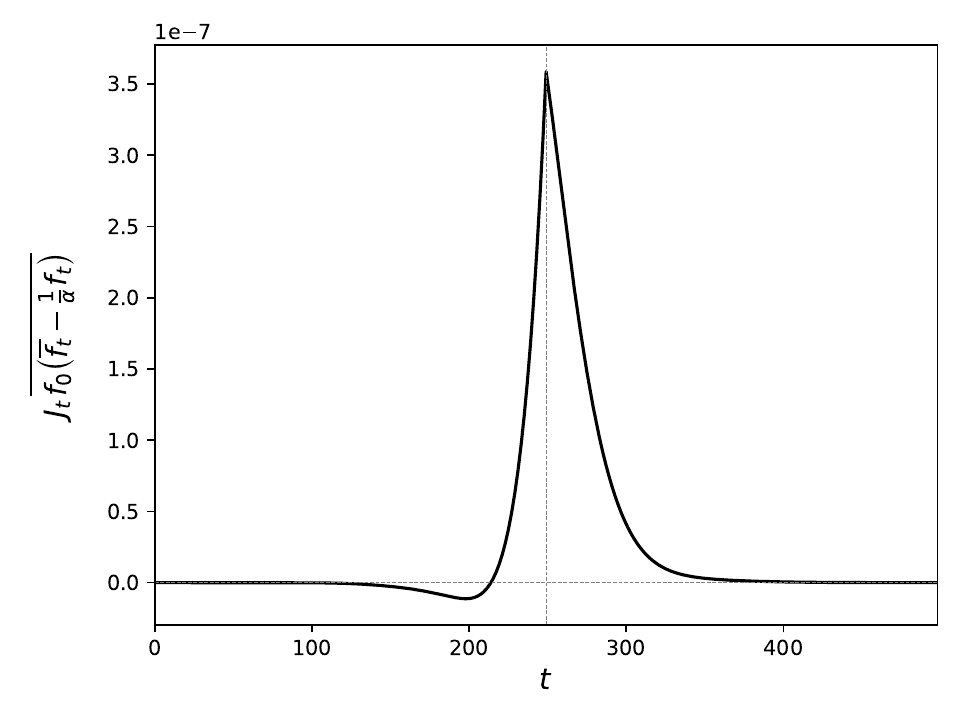}
    \includegraphics[width=0.32\linewidth]{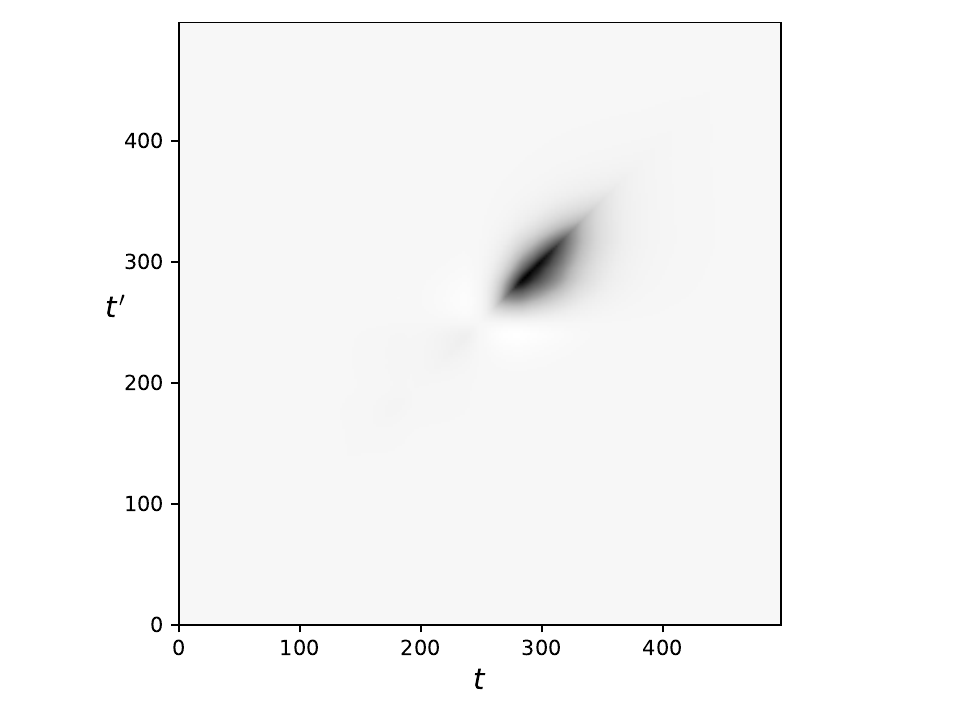}
    \includegraphics[width=0.32\linewidth]{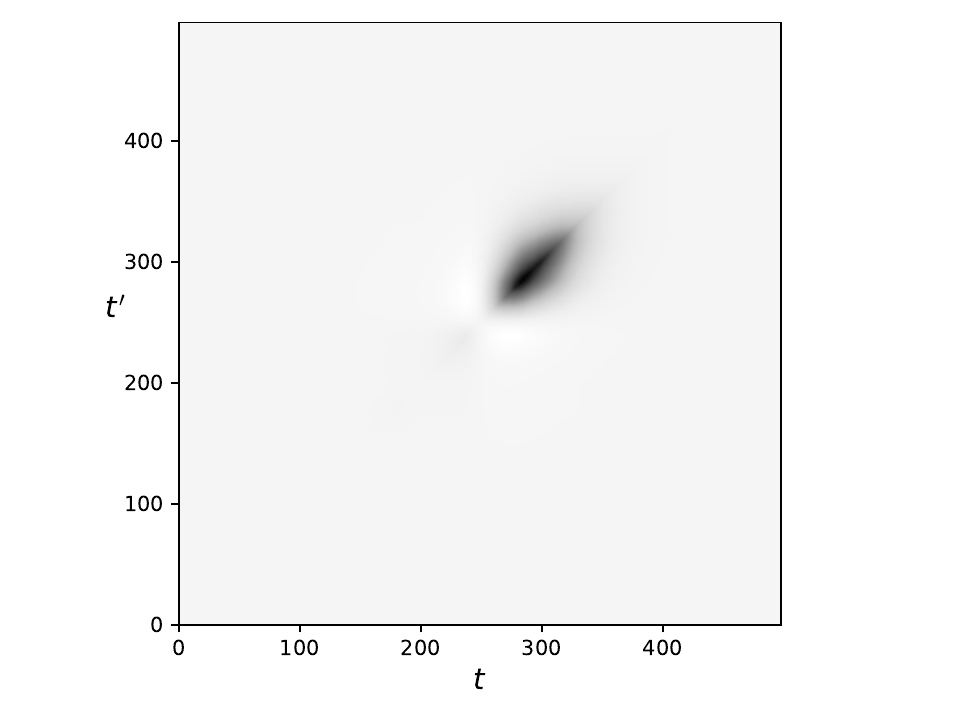}
    \includegraphics[width=0.32\linewidth]{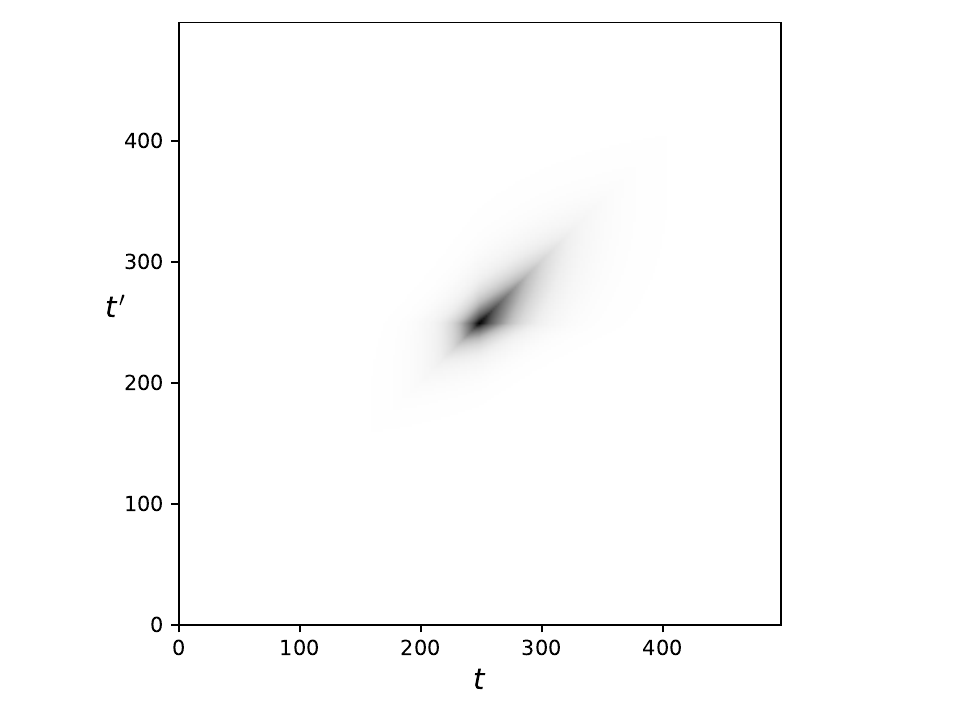}
    \caption{Illustration of the path correction integrals of Eq. \eqref{variance path corrections} and Eq. \eqref{path impact on expectation}, in the numerical experiment introduced in the main text Fig. (1). They are respectively, from the left: (above)  $ J_{t} \,f^{t}$, $ J_{t} \,\overline{f^{t}}$, and $
     J_{t} \, \overline{f_0 \left(\overline{f^{t}} -\frac{1}{\alpha}f^{t} \right)} $; (below) $K^{(1)}_{t, t'} f^{t} f^{t'}$, $K^{(2)}_{t, t'} f^{t} f^{t'}$, and $K_{t, t'}\, \overline{f^{t} f^{t'}}$.}
    \label{fig:3_2_scaling}
\end{figure}

\section{Derivation of Eq. (16)}

Let us first note that the fluctuation theorem of Eq. \eqref{fluctuation theorem} is violated when the ML path is not a constant, meaning $f_t\neq 0$, because it introduces as a space-dependent coefficient for the Langevin dynamics $\partial_u x_{t, u} -\eta_{t, u} = \frac{1}{\sigma^2} \partial^2_t x_{t, u} -(\alpha +f_t) (e^{x_{t, u}} -1)$, therefore the 
homogeneity of expectations is broken, $p(\widetilde{x}_{t, u}) \neq p(\widetilde{x}_{0, 0})$.
Then the first moment $\langle x\rangle$ is not a simple function of the higher order moments like in the homogeneous case.
Let us then consider the perturbation expansion,
\begin{multline}
    x_{0, 0} = y_{0, 0} - G_{-t, -u} \left\{ \alpha \left[ \exp\left(x^{t,u}\right) -1^{t,u} -x^{t,u} \right]  + f^{t} \left[ \exp\left(x^{t,u}\right) -1^{t,u} \right]  \right \} \\
    = y_{0, 0} - G^{-t, -u} \left\{ \frac{\alpha}{2} \left[ x_{t,u}^2 +\frac{1}{3} \widetilde{x}_{t,u}^3 +\frac{1}{12} y_{t,u}^4  \right]  + f_{t} \left[ x_{t,u} +\frac{1}{2} x_{t,u}^2 \right]  \right\} +\mathcal{O}(y^5) +\mathcal{O}(y^3 f) \\
    = y_{0, 0} - \frac{\alpha}{2} G^{-t, -u} \Bigg\{ \frac{1}{3} \widetilde{x}_{t, u}^3 +\frac{1}{12} y_{t, u}^4 \\
    +\left[ y_{t, u} - \frac{\alpha}{2} G_{t-t', u-u'} \left( \{ \widetilde{x}^{t', u'}\}^2 + \frac{1}{3} \{y^{t', u'}\}^3 \right) 
    -G_{t-t', u-u'} f^{t'} \left( y^{t', u'} -G^{t'-t'', u'-u''} f_{t''} y_{t'', u''} \right)
    \right]^2  \Bigg\} \\
    - G^{-t, -u} f_t \Bigg\{ y_{t, u} -  \frac{\alpha}{2} G_{t-t', u-u'} \left( y^{t', u'} -G^{t'-t'', u'-u''} f_{t''} y_{t'', u''} \right)^2 \\
    -G_{t-t', u-u'} f^{t'} \left[ y^{t', u'} -\frac{\alpha}{2}G^{t'-t'', u'-u''} y_{t'', u''}^2 +\frac{1}{2} (y^{t', u'})^2 \right]
    +\frac{1}{2} \left( y_{t, u} -G_{t-t', u-u'} f^{t'} y^{t', u'} \right)^2 \Bigg\} \\
    +\mathcal{O}(y^5) +\mathcal{O}(y^3 f) +\mathcal{O}(y^2 f^3) +\mathcal{O}(y f^3) \\
    = \widetilde{x}_{0, 0} - \frac{\alpha}{2} G^{-t, -u} \left[ -2 y_{t, u} G_{t-t', u-u'} f^{t'} \left( y^{t', u'} -G^{t'-t'', u'-u''} f_{t''} y_{t'', u''} \right) +G_{t-t', u-u'} f^{t'} y^{t', u'} G_{t-t'', u-u''} f^{t''} y^{t'', u''} \right] \\
    - G^{-t, -u} f_t \Bigg\{ -  \frac{\alpha}{2} G_{t-t', u-u'} \left[ ( y^{t', u'})^2 -2y^{t', u'}G^{t'-t'', u'-u''} f_{t''} y_{t'', u''} \ \right] \\
    -G_{t-t', u-u'} f^{t'} \left[ -\frac{\alpha}{2}G^{t'-t'', u'-u''} y_{t'', u''}^2 +\frac{1}{2} (y^{t', u'})^2 \right]
    +\frac{1}{2} \left( y_{t, u}^2 -2y_{t, u}G_{t-t', u-u'} f^{t'} y^{t', u'} \right) \Bigg\} \\
    +\mathcal{O}(y^5) +\mathcal{O}(y^3 f) +\mathcal{O}(y^2 f^3) +\mathcal{O}(y f^3) ,
\end{multline}
where terms of order $\mathcal{O}(y^3 f)$ and $\mathcal{O}(y f)$ are not considered as they will vanish when taking the Gaussian expectation, while terms of order $\mathcal{O}(y^2 f^3)$ are not considered because they are regarded as statistically the same order of $\mathcal{O}(y^5)$ according to the scaling logic of Eq. \eqref{f sim y}.
Taking the Gaussian expectations we find
\begin{multline}
    \langle x_{0, 0} \rangle -  \langle \widetilde{x}_{0, 0} \rangle +\mathcal{O}\left(\langle y^2\rangle ^{5/2}\right)\\
    = - \frac{\alpha}{2} G^{-t, -u} \left[ -2 G_{t-t', u-u'} f^{t'} \left( C^{t-t', u-u'} -G^{t'-t'', u'-u''} f_{t''} C_{t-t'', u-u''} \right) +G_{t-t', u-u'} f^{t'} G_{t-t'', u-u''} f^{t''} C^{t''-t', u''-u'} \right] \\
    - G^{-t, -u} f_t \Bigg[ -  \frac{\alpha}{2} G_{t-t', u-u'} \left( \langle y^2 \rangle 1^{t', u'} -2 G^{t'-t'', u'-u''} f_{t''} C_{t'-t'', u'-u''} \right) \\ - G_{t-t', u-u'} f^{t'} \langle y^2 \rangle \left( -\frac{\alpha}{2} G^{t'-t'', u'-u''}  1_{t'', u''} +\frac{1^{t', u'}}{2} \right)
    +\frac{1}{2} \left(  \langle y^2\rangle 1_{t, u} -2 G_{t-t', u-u'} f^{t'} C^{t'-t, u'-u} \right) \Bigg] 
    \\
    = - \frac{\alpha}{2} G^{-t, -u} \Bigg[ -2 G_{t-t', u-u'} f^{t'} \left( C^{t-t', u-u'} -G^{t'-t'', u'-u''} f_{t''} C_{t-t'', u-u''} \right) +G_{t-t', u-u'} f^{t'} G_{t-t'', u-u''} f^{t''} C^{t''-t', u''-u'} \\
    +2 G_{t-t', u-u'} G^{t'-t'', u'-u''} f_{t''} C_{t'-t'', u'-u''} f_t  -2 G_{t-t', u-u'} C^{t'-t, u'-u} \frac{f_t f^{t'}}{\alpha} \Bigg] 
    \\
    = - \frac{\alpha}{2} G^{-t, -u} 1_{u} \Bigg[ -2 G_{-t', -u'} f_{t+t'} \left( C^{-t', -u'} -G^{t'-t'', u'-u''} f_{t+t''} C_{-t'', -u''} \right) +G_{-t', -u'} f_{t+t'} G_{-t'', -u''} f_{t+t''} C^{t''-t', u''-u'} \\
    +2 G_{-t', -u'} G^{t'-t'', u'-u''} f_{t+t''} C_{t'-t'', u'-u''} f_t  -2 G_{-t', -u'} C^{t', u'} \frac{f_t f_{t+t'}}{\alpha} \Bigg],
\end{multline}
where we have used the identity $G_{t,u} 1^{t,u} = 1/\alpha$, and in the last passage transformed the integration coordinates to $\widetilde{t'} = t'-t$, $\widetilde{t''} = t''-t$, $\widetilde{u'} = u'-u$, and $\widetilde{u''} = u''-u$.
Using the definitions of Eqs. \eqref{def J}-\eqref{def K} we rewrite this as
\begin{multline}
    \langle x_{0, 0} \rangle -  \langle \widetilde{x}_{0, 0} \rangle +\mathcal{O}\left(\langle y^2\rangle ^{5/2}\right) \\
    = - \frac{\alpha}{2} G^{-t, -u} 1_u \left[ J^{t'} f_{t+t'} \left(1+\frac{f_t}{\alpha}\right) +K^{t', t''} f_{t+t'} f_{t+t''}
    - G_{-t', -u'} 1^{u'} J^{t'-t''} f_{t+t''} f_t  \right] \\
    = - \frac{\alpha}{2} G^{-t, -u} 1_u \left[ J^{t'} f_{t+t'} +K^{t', t''} f_{t+t'} f_{t+t''}
    - f_t J^{t'} \left(G^{-t'', -u''} 1_{u''}f_{t+t'+t''} -\frac{1}{\alpha}f_{t+t'} \right)   \right] ,
\end{multline}
where we changed variables in
\begin{equation}
    G_{-t', -u'} 1^{u'} J^{t'-t''} f_{t+t''} = G^{-t', -u'} 1_{u'} J^{t''} f_{t+t'+t''} = G^{-t'', -u''} 1_{u''} J^{t'} f_{t+t'+t''} .
\end{equation}
Let us now define the smoothed path as
\begin{equation}
    \overline{f_t} \equiv G^{-t', -u'} 1_{u'} f_{t+t'} = \langle y^2 \rangle \int dt' \, e^{-t'/\tau} f_{t+t'},
\end{equation}
and similarly the smoothed product is
\begin{equation}
    \overline{f_t f_{t'}} \equiv G^{-t'', -u''} 1_{u''} f_{t+t''} f_{t'+t''} = \langle y^2 \rangle \int dt'' \, e^{-t''/\tau} f_{t+t''}f_{t'+t''},
\end{equation}
and we recall that the timescale is $\tau\equiv 1/(\sigma \sqrt{\alpha})$, and the Gaussian variance is $\langle y^2 \rangle = \sigma/(2\sqrt{\alpha})$.
In terms of the smoothed observables the path impact on the expectation is rewritten as
\begin{equation}\label{path impact on expectation}
    \langle x_{0, 0} \rangle -  \langle \widetilde{x}_{0, 0} \rangle 
    = - \frac{\alpha}{2} \left[ J_{t} \,\overline{f^{t}} +K_{t, t'}\, \overline{f^{t} f^{t'}}
    - J_{t} \, \overline{f_0 \left(\overline{f^{t}} -\frac{1}{\alpha}f^{t} \right)}   \right] 
    +\mathcal{O}\left(\langle y^2\rangle ^{5/2}\right) ,
\end{equation}
and we recall that $\langle \widetilde{x}_{0, 0} \rangle = -\frac{1}{2}\langle y^2 \rangle$ from Eq. \eqref{tilde mu}.

The skewness correction of Eq. \eqref{tilde skew} is already of order $\mathcal{O}(\langle y^2 \rangle^2)$, therefore path impacts do not appear at this order, and the same applies for all the other higher order cumulants. The first two moments are then the only impacted by the path $f_t$, and they are given by Eq. \eqref{path impact on expectation} and Eq. \eqref{variance path corrections}, based on the definitions of $J_t$ and $K_{t, t'}$, see Eqs. \eqref{def J}-\eqref{def K}.
Let us define as $p_G(x_0)=\mathcal{G}(0, \langle y^2 \rangle)$ the reference Gaussian density where $\langle y^2 \rangle=\sigma/(2\sqrt{\alpha})$.
To test our perturbative approach to evaluate the path impact on the true density $p(x_0)$, we estimate the probability displacement $\delta p\equiv p(x_0)-p_G(x_0)$ with direct numerical simulations of the SPDE, and compare it with the Gram-Charlier expansion of Eq. \eqref{Gram–Charlier} based on the moments predicted by the perturbative expansion.
For the sake of visualization we also consider the displacement from the corresponding homogeneous $f_t = 0$ case $\widetilde{\delta p}\equiv p(\widetilde{x}_0)-p_G(x_0)$. 
The Python implementation of the numerical testing framework is available at \textit{github.com/AndreaAuconi/BayesianFieldTheory}.

\begin{figure}
    \centering    \foreach \i in {one, two, three, four, nine} {
    \includegraphics[width=0.32\linewidth]{SM_plots/\i_ML.pdf} \hfill
    \includegraphics[width=0.32\linewidth]{SM_plots/\i_numerical_path_impact.pdf}
    \includegraphics[width=0.32\linewidth]{SM_plots/\i_numerical_path_only.pdf}
}
    \caption{Additional examples from the numerical testing framework introduced in the main text for the derived perturbative corrections. The parameters are $\sigma = 0.02$ and $\alpha \approx r_0 = 1$. On the left is the ML curve and underlying process, in the center the simulated and theoretical distribution displacement $\delta p$ relative the local Gaussian solution, and on the right the same plot but subtracting the homogeneous $f_t=0$ case as $\delta p-\widetilde{\delta p}$. Note that in the absence of a strong shape correction the estimation of $\delta p-\widetilde{\delta p}$ is dominated by numerical noise. The Python implementation is available at \textit{github.com/AndreaAuconi/BayesianFieldTheory}.}
    \label{fig:examples}
\end{figure}

\begin{figure}
    \centering    \foreach \i in {six,seven,eight,ten} {
    \includegraphics[width=0.32\linewidth]{SM_plots/\i_ML.pdf} \hfill
    \includegraphics[width=0.32\linewidth]{SM_plots/\i_numerical_path_impact.pdf}
    \includegraphics[width=0.32\linewidth]{SM_plots/\i_numerical_path_only.pdf}
}
\includegraphics[width=0.32\linewidth]{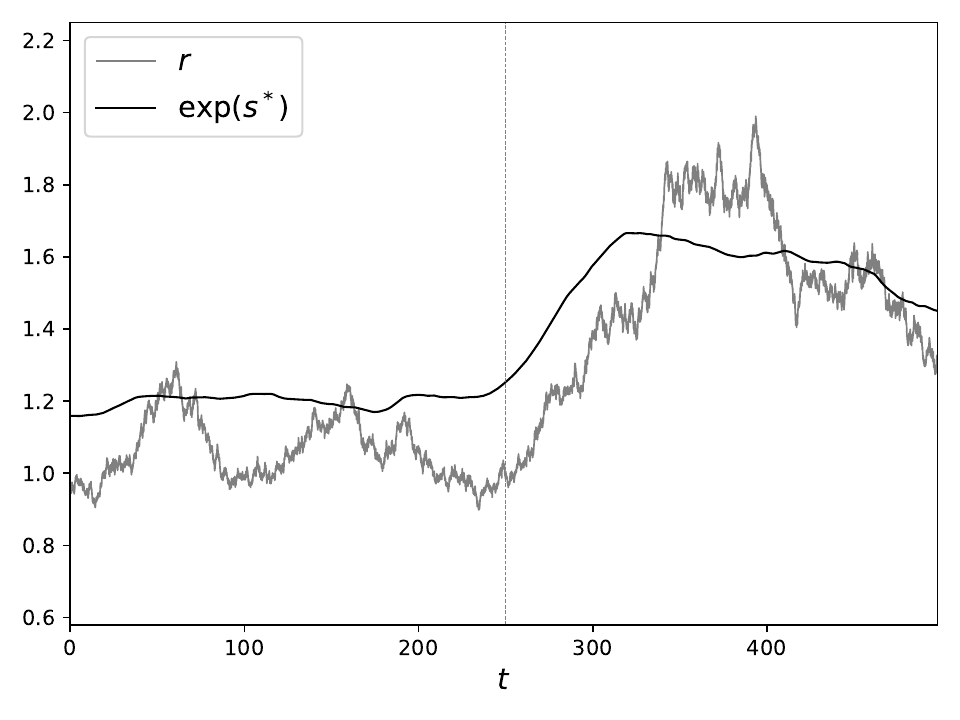} \hfill
    \includegraphics[width=0.32\linewidth]{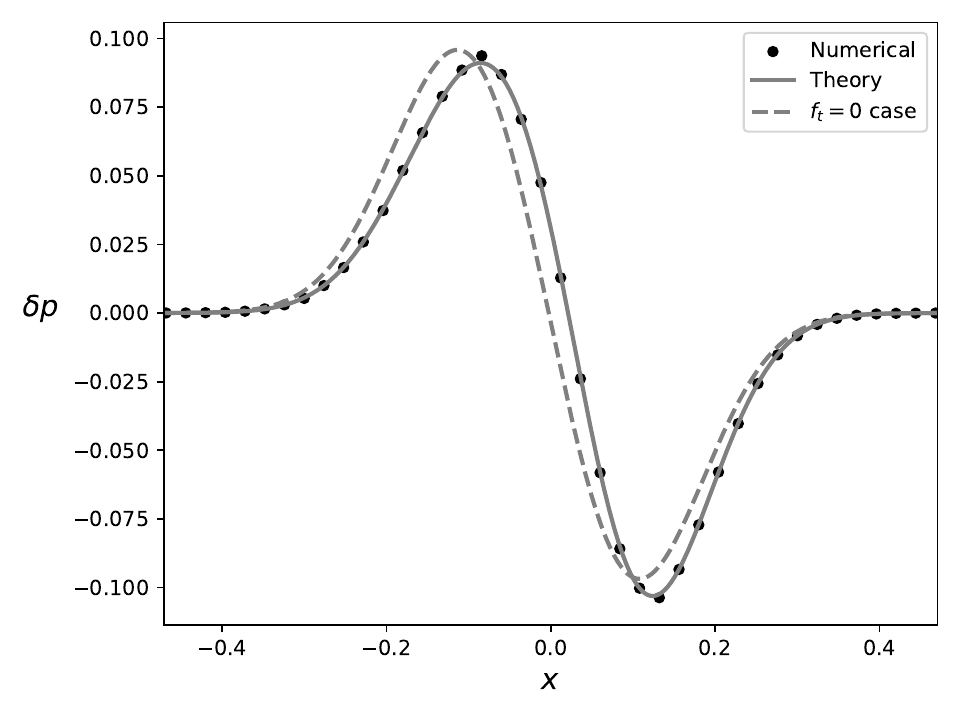}
    \includegraphics[width=0.32\linewidth]{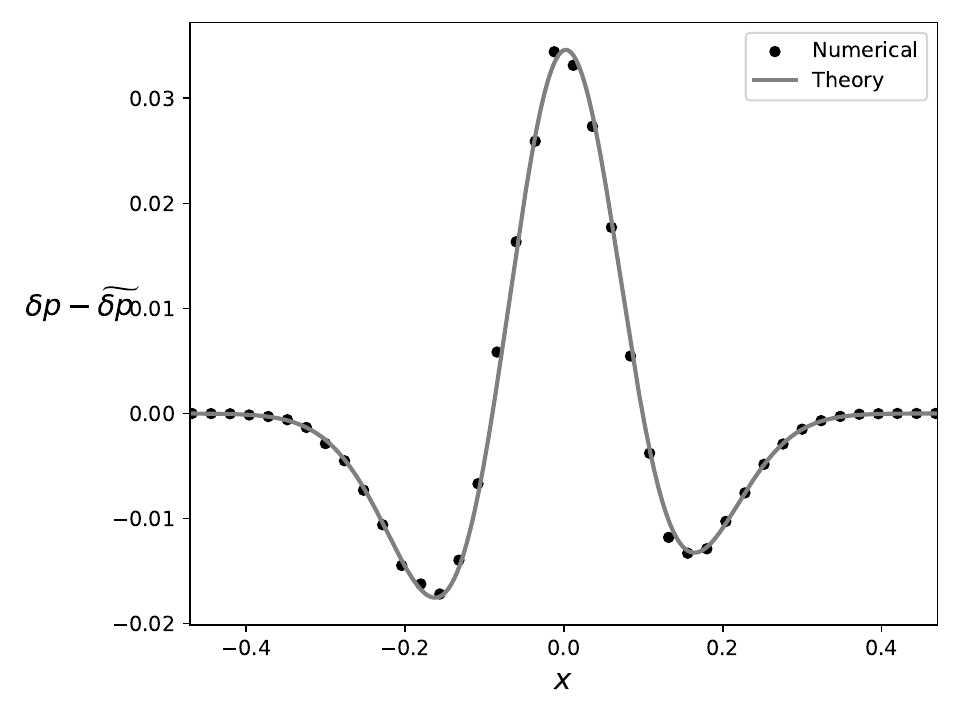}
    \caption{More examples like Fig. \ref{fig:examples}. The last row is the one presented in the main text.}
    \label{fig:more_examples}
\end{figure}

\section{The $K_{t, t'}$ integral}

Let us consider the two terms in Eq. \eqref{def K} separately, $K_{t, t'} = K^{(1)}_{t, t'} +K^{(2)}_{t, t'}$. The first term is
\begin{multline}
     K^{(1)}_{t, t'} \equiv 2 G_{-t, -u} {G_{t-t',}}^{u-u'} C_{t', u'}
   \\ = \frac{\sigma^3}{4 \pi^2} \int  \frac{dk}{\alpha +k^2} \cos(k \sigma t')  \int_{-\infty}^0 \frac{du}{\sqrt{-u}} \exp \left( \frac{\sigma^2 t^2}{4 u} \right)  \int_{-\infty}^u \frac{du'}{\sqrt{(u-u')}} \exp \left[ (2\alpha+k^2) u' - \frac{\sigma^2 (t-t')^2}{4 (u-u')} \right] 
   \\
   = \frac{\sigma^3}{4 \pi^2} \int  \frac{dk}{\alpha +k^2} \cos(k \sigma t')  \int_{-\infty}^0 \frac{du}{\sqrt{-u}} \exp \left[ \frac{\sigma^2 t^2}{4 u} + (2\alpha+k^2) u \right] \int_{0}^{\infty} \frac{dv}{\sqrt{v}} \exp \left[ -(2\alpha+k^2) v - \frac{\sigma^2 (t-t')^2}{4 v} \right] 
   \\
   = \frac{\sigma^3}{4 \pi^{3/2}} \int  \frac{dk}{(\alpha +k^2)\sqrt{2\alpha +k^2}} \cos(k \sigma t') \exp \left(-\sigma |t-t'| \sqrt{2\alpha +k^2} \right)  \int_{-\infty}^0 \frac{du}{\sqrt{-u}} \exp \left[ \frac{\sigma^2 t^2}{4 u} + (2\alpha+k^2) u \right]
   \\
   = \frac{\sigma^3}{4 \pi} \int \frac{dk}{(\alpha +k^2)(2\alpha +k^2)} \cos(k \sigma t') \exp \left[-\sigma \left(|t-t'| +|t|\right) \sqrt{2\alpha +k^2} \right]
    \\
   = \langle y^2 \rangle^3 \frac{2}{\pi} \int \frac{dk}{(1 +k^2)(2 +k^2)} \cos\left(k \frac{t'}{\tau}\right) \exp \left[-\left(\frac{|t-t'| +|t|}{\tau}\right) \sqrt{2 +k^2} \right] ,
\end{multline}
where we again used the integral $\int_0^{\infty} dx\, e^{-\gamma x -\beta/x} x^{-1/2} = \sqrt{\pi/\gamma}\, e^{-2\sqrt{\beta \gamma}} $ (with $\beta>0$, $\gamma>0$) from Ref. \cite{gradshteyn2014table} (7th Ed., pg. 369).
The second term is
\begin{multline}
    K^{(2)}_{t, t'} \equiv  G_{-t, -u}G_{-t', -u'} {C_{t-t',}}^{u-u'}\\
    = \frac{\sigma^3}{8 \pi^2} \int \frac{dk}{\alpha +k^2} \cos[k \sigma (t-t')] \iint_{-\infty}^0 \frac{du\, du'}{\sqrt{u u'}} \exp \left[ \alpha (u+u') + \frac{\sigma^2 t^2}{4 u} + \frac{\sigma^2 t'^2}{4 u'} -(\alpha+k^2) | u-u' | \right]
    \\
    = \langle y^2 \rangle^3 \frac{1}{\pi^2} \int \frac{dk}{1 +k^2} \cos\left[k \frac{(t-t')}{\tau}\right] \iint_{0}^{\infty} \frac{du\, du'}{\sqrt{u u'}} \exp \left[ -u-u' - \frac{1}{4u}\left(\frac{t}{\tau} \right)^2 - \frac{1}{4u'}\left(\frac{t'}{\tau} \right)^2 -(1+k^2) | u-u' | \right]
    \\
    = \langle y^2 \rangle^3 \frac{1}{\pi^3} \iint \frac{dk\,dk'}{{k'}^2 + (1+k^2)^2} \cos\left[k \frac{(t-t')}{\tau}\right] \iint_{0}^{\infty} \frac{du\, du'}{\sqrt{u u'}} \exp \left[ -(1-ik')u-(1+ik')u' - \frac{1}{4u}\left(\frac{t}{\tau} \right)^2 - \frac{1}{4u'}\left(\frac{t'}{\tau} \right)^2 \right]
    \\
    = \langle y^2 \rangle^3 \frac{1}{\pi^2} \iint \frac{dk\,dk'}{\sqrt{1+{k'}^2} \left[{k'}^2 + (1+k^2)^2\right]} \cos\left[k \frac{(t-t')}{\tau}\right]  \exp \left[ -\frac{|t|}{\tau} \sqrt{1-ik'} -\frac{|t'|}{\tau} \sqrt{1+ik'} \right]
    ,
\end{multline}
where we used the Fourier representation $\exp(-a|x|)= (a/\pi) \int dk\, (a^2 +k^2)^{-1} \exp(ikx)$ to factorize the integrals in $du$ and $du'$, which are again of the form $\int_0^{\infty} dx\, e^{-\gamma x -\beta/x} x^{-1/2} = \sqrt{\pi/\gamma}\, e^{-2\sqrt{\beta \gamma}} $, and by definition we are considering the principal branch in the imaginary square roots, meaning $Re\left[\sqrt{1-ik'}\right]>0$ and $Re\left[\sqrt{1+ik'}\right]>0$.
These are given by
\begin{equation}
    \sqrt{1\pm ik'} = \sqrt{\frac{\sqrt{1+k'^2} +1}{2}} 
    \pm i \sign (k') \sqrt{\frac{\sqrt{1+k'^2} -1}{2}} .
\end{equation}
Of the phase part, by symmetry we see that the odd sine term vanishes under the $dk'$ integral, so we obtain
\begin{multline}
    K^{(2)}_{t, t'} = \langle y^2 \rangle^3 \frac{1}{\pi^2} \iint \frac{dk\,dk'}{\sqrt{1+{k'}^2} \left[{k'}^2 + (1+k^2)^2\right]} \cos\left[k \frac{(t-t')}{\tau}\right]  \\
    \times \exp \left[ -\frac{(|t|+|t'|)}{\tau} \sqrt{\frac{\sqrt{1+k'^2} +1}{2}} \right]
    \cos \left[ \frac{(|t|-|t'|)}{\tau} \sqrt{\frac{\sqrt{1+k'^2} -1}{2}} \right],
\end{multline}
where the $\sign (k')$ factor in the cosine argument was removed by symmetry.
The solution to the $dk$ integral is provided in Ref. \cite{gradshteyn2014table} (7th Ed., pg. 428),
\begin{multline}
    \int \frac{dk}{\left[{k'}^2 + (1+k^2)^2\right]} \cos\left[k \frac{(t-t')}{\tau}\right]
    = \frac{\pi}{|k'|\sqrt{1+{k'}^2}} \exp \left( -\frac{|t-t'|}{\tau} \sqrt{\frac{\sqrt{1+k'^2} +1}{2}} \right)
    \\
    \times \left[ \sqrt{\frac{\sqrt{1+k'^2} -1}{2}} \cos \left( \frac{|t-t'|}{\tau} \sqrt{\frac{\sqrt{1+k'^2} -1}{2}} \right) +\sqrt{\frac{\sqrt{1+k'^2} +1}{2}} \sin \left( \frac{|t-t'|}{\tau} \sqrt{\frac{\sqrt{1+k'^2} -1}{2}} \right) \right] .
\end{multline}
The resulting $dk'$ integral, noting again that by symmetry the odd sine term vanishes, reads
\begin{multline}
    K^{(2)}_{t, t'} = \langle y^2 \rangle^3 \frac{1}{\pi} \int \frac{dk'}{|k'| (1+{k'}^2)} \sqrt{\frac{\sqrt{1+k'^2} -1}{2}}  \exp \left[ -\frac{(|t-t'|+|t|+|t'|)}{\tau} \sqrt{\frac{\sqrt{1+k'^2} +1}{2}} \right] \\
    \times
    \cos \left[ \frac{(|t|-|t'|)}{\tau} \sqrt{\frac{\sqrt{1+k'^2} -1}{2}} \right]  \cos \left( \frac{|t-t'|}{\tau} \sqrt{\frac{\sqrt{1+k'^2} -1}{2}} \right) .
\end{multline}

\section{Neuron data analysis}

The analysis was performed on single-unit recordings obtained from the Allen Brain Observatory using the AllenSDK \textit{allensdk.readthedocs.io/en/latest/}.
To ensure the reliability of the rate estimation, we filtered for neurons satisfying strict stability requirements, specifically an Inter-Spike Interval (ISI) violations score of less than 0.5 and a presence ratio greater than 0.9.
Candidates passing the quality control were sorted hierarchically, prioritizing first the presence ratio (descending) to maximize stability, and second the firing rate (descending) to ensure sufficient data volume.
The top five neurons resulting from this ranking were extracted and stored for detailed analysis.

For each selected neuron, the spike times were extracted, and the analysis window $[T_i, T_f]$ was defined relative to the recorded spike train to cover a representative fraction of the data, only limited by our computational resources.
The estimation of the volatility parameter $\sigma$, which governs the stochastic dynamics of the rate according to the minimal GBM model, was performed using the Bayesian evidence framework introduced above in Eq. \eqref{evidence Bayes} and evaluated with the Laplace approximation. 
The maximum posterior $\sigma^*$ was then selected and fixed as a constant for this illustrative application, meaning that the impact of the uncertainty $p(\sigma|D)$ was not studied.
The reconstructed $\sigma^*$ and corresponding reconstructed trajectories and uncertainties for the first two neurons (at selected time intervals) are shown in Fig. (\ref{fig:SM_neuron}).
The Python implementation is available at \textit{github.com/AndreaAuconi/BayesianFieldTheory}.

\begin{figure}
    \centering    \includegraphics[width=0.3\linewidth]{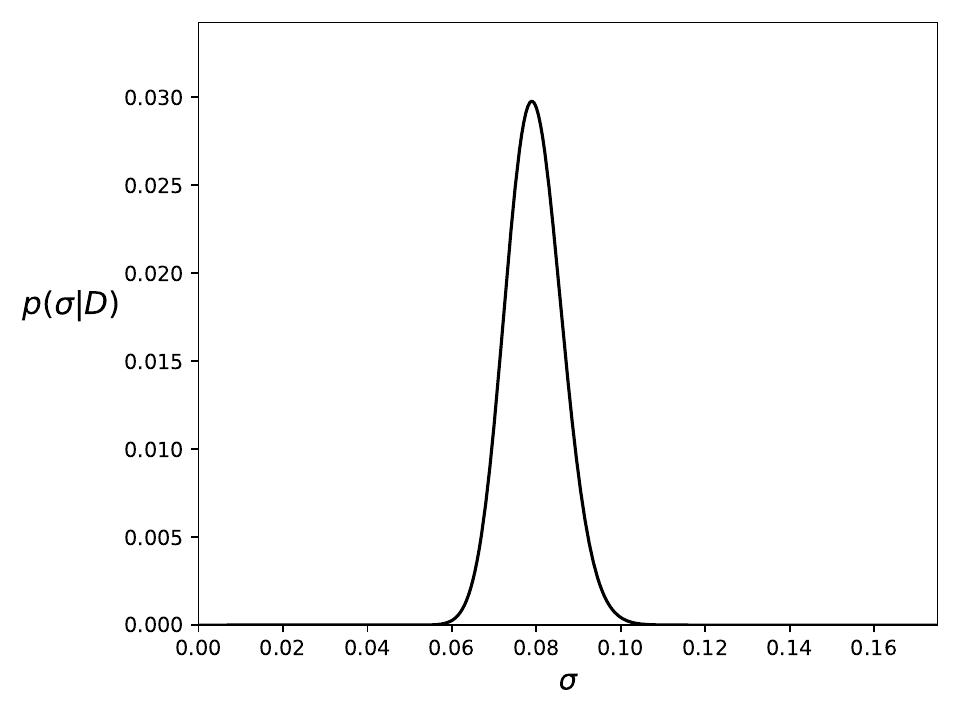}
    \includegraphics[width=0.3\textwidth]{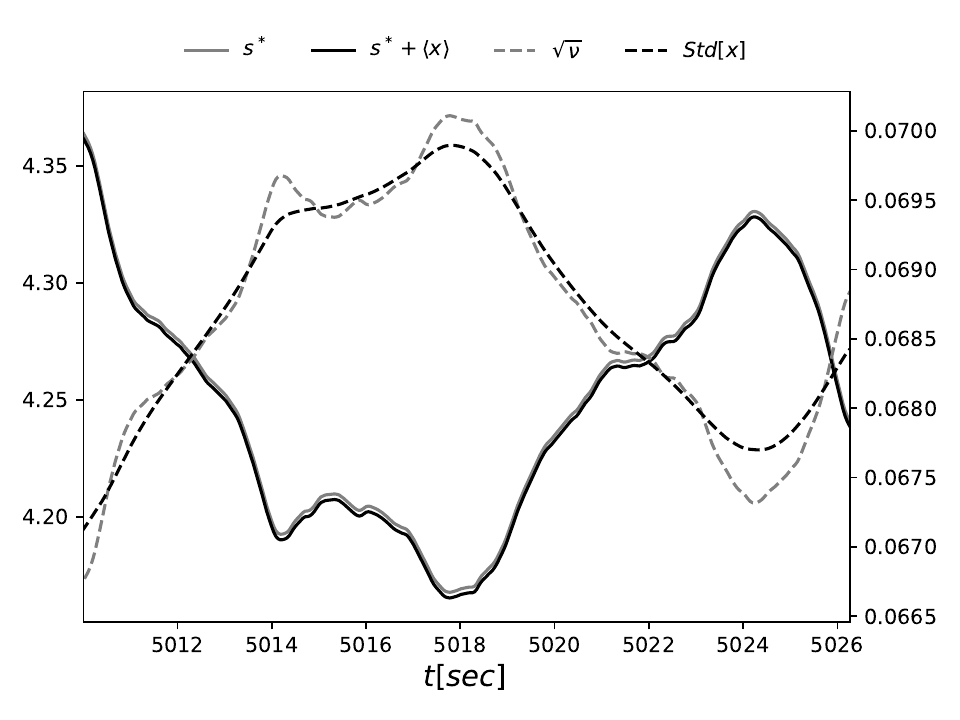}
    \includegraphics[width=0.3\textwidth]{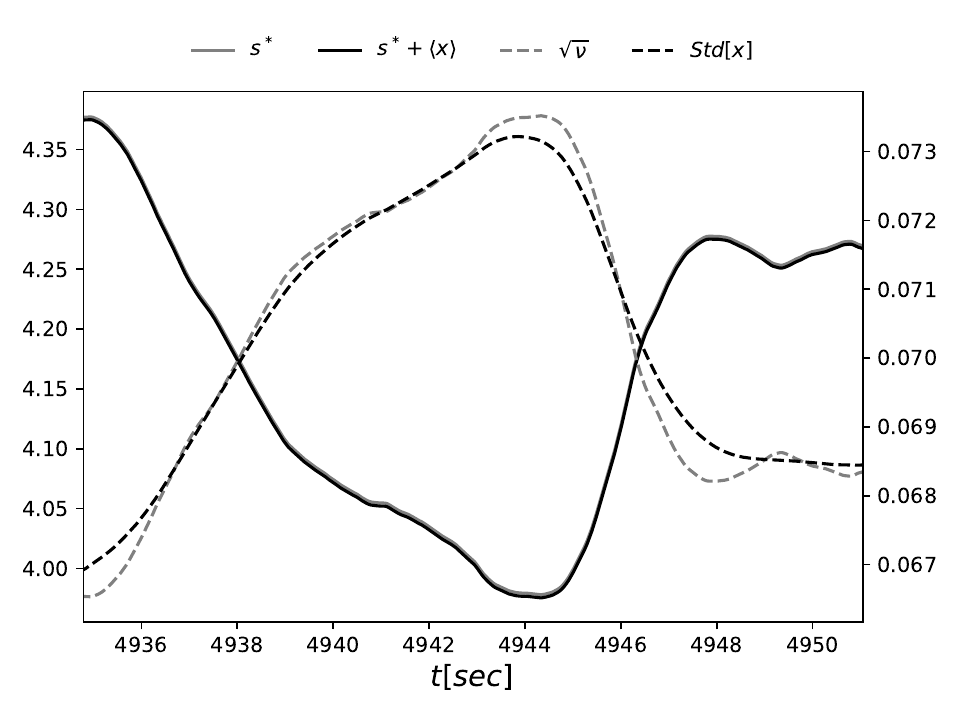}
    \includegraphics[width=0.3\linewidth]{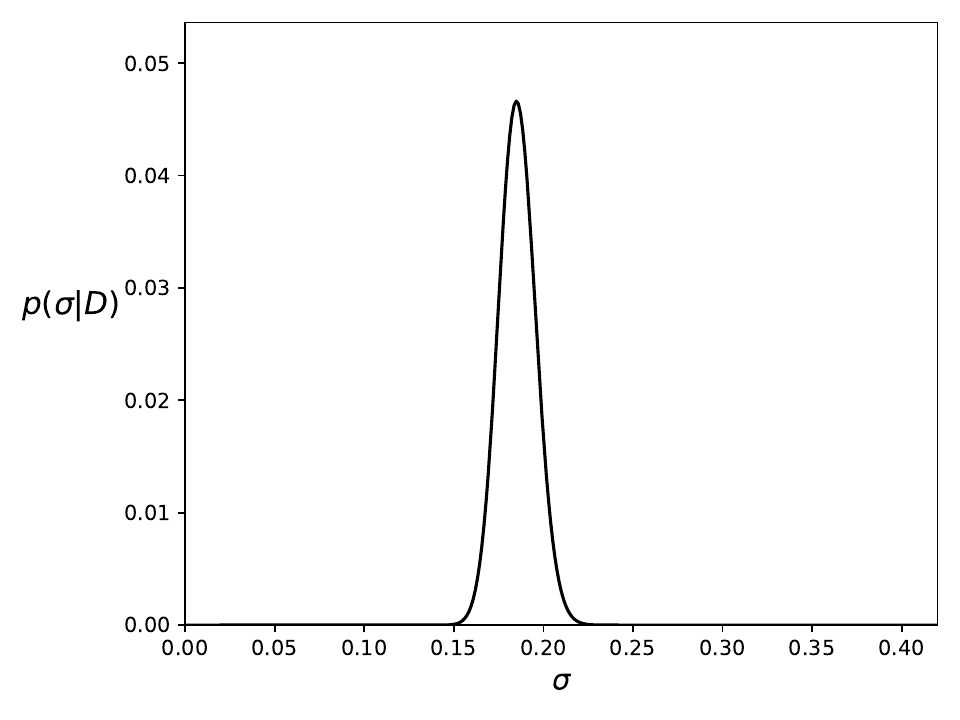}
    \includegraphics[width=0.3\textwidth]{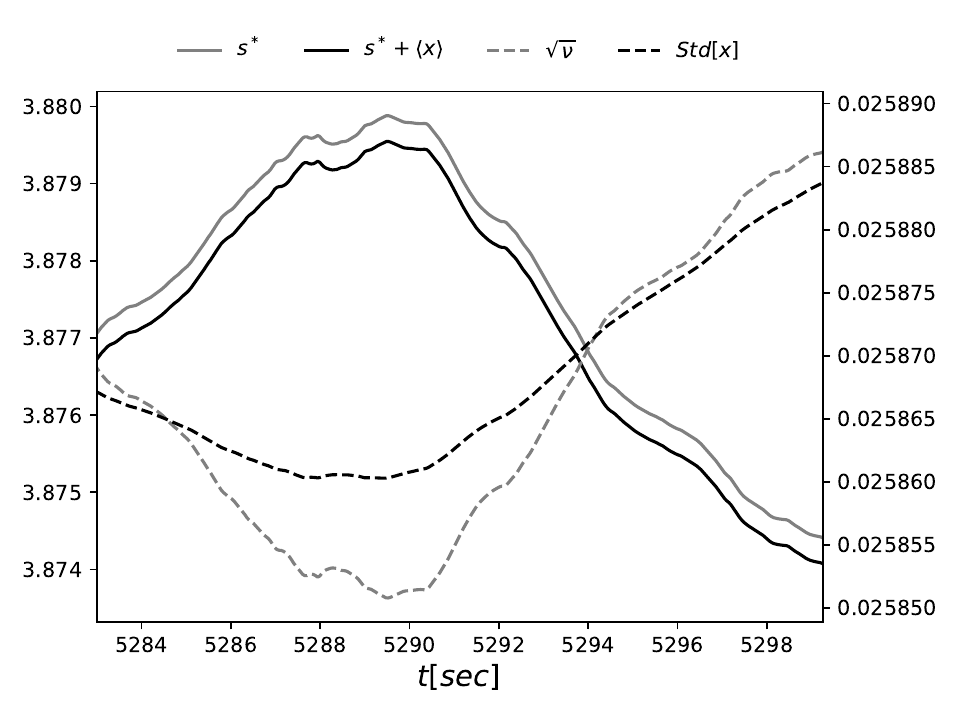}
    \includegraphics[width=0.3\textwidth]{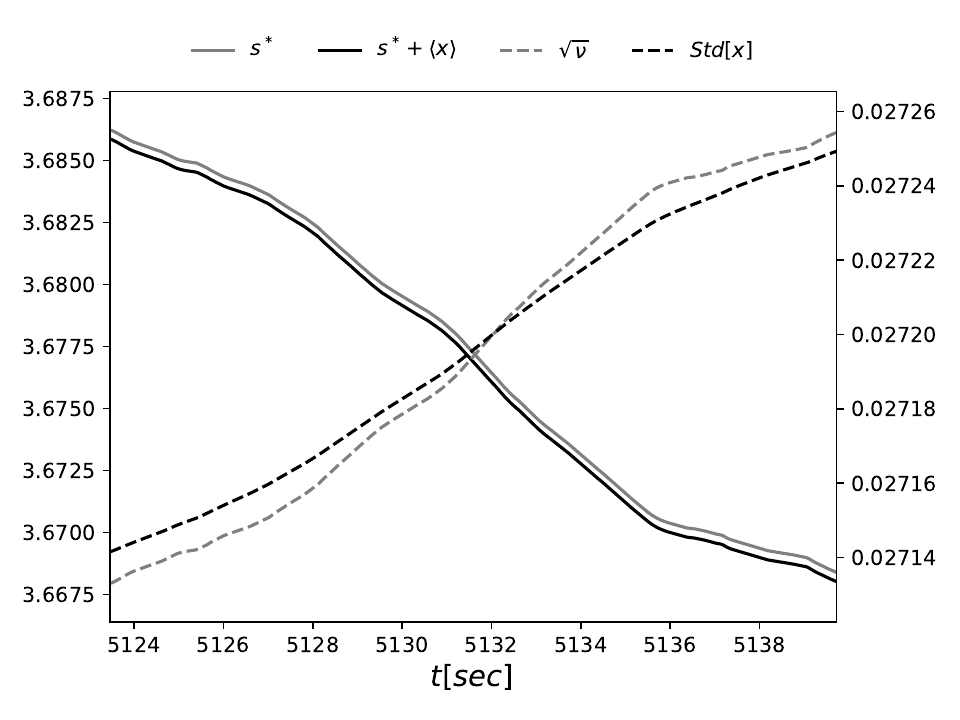}
    \caption{Posterior distribution $p(\sigma|D)$ of the volatility parameter computed via the saddle-point approximation scan, and two examples of the rate reconstruction (at the maximum likelihood volatility $\sigma^* = argmax_\sigma p(\sigma|D)$ for illustrative purposes) according to the local Gaussian regime (in gray) and to perturbative expansion $\mathcal{O}(\nu^2)$ (in black), for the two neurons under study.
    }
    \label{fig:SM_neuron}
\end{figure}

\bibliography{bibliography}% Produces the bibliography via BibTeX.

\end{document}
